# Supplementary material for: How Does Supernet Help in Neural Architecture Search?
Source: arXiv:2010.08219 source file (2021-05-05)
Supplement: Supplementary file 1 [file appendix.tex]

\appendix

\section{Experiment Setups}

\subsection{Hyper-Parameter Settings}

We list the hyper-parameters we used in supernet training in \autoref{tab:hparams-supernet}.

\begin{table}[h]
    \centering
    \caption{Summary of hyper-parameters used in supernet training. For batch size marked with stars, we use a \emph{multi-path parallel strategy} that samples different architectures on different GPUs within a same mini-batch. BN calib batch size / steps~\cite{bender18understanding} are the configuration of batch-norm calibration before evaluation of each architecture.}
    \label{tab:hparams-supernet}
    \begin{tabular}{c|c|c|c|c|c}
    \hline
    & NB-101 & NB-201 & DARTS-C & Proxyless & DARTS-P \\
    \hline
    Batch size & 256 & 256 & 448$^*$ & 1024$^*$ & 256 \\
    Initial LR & 0.1 & 0.05 & 0.1 & 0.2 & 40 \\
    LR Decay   & Cosine & Cosine & Cosine & Cosine & Fixed \\
    Ending LR  & 0 & 0 & 0 & 0 & 40 \\
    Optimizer  & SGD & SGD & SGD & SGD & SGD/ASGD \\
    Momentum   & 0.9 & 0.9 & 0.9 & 0.9 & 0 \\
    Nesterov   & no  & yes & no  & no  & no \\
    Weight decay & 0.0001 & 0.0005 & 0.0003 & 0.0005 & $8 \cdot 10^7$ \\
    % Initial convolution filters & 128 & 16 & 36 & 40 & - \\
    Gradient clip & 5 & 5 & 5 & 0 & 0.1 \\
    Auxiliary weight & 0 & 0 & 0.4 & 0 & - \\
    Label smoothing~\cite{szegedy2016rethinking} & 0 & 0 & 0 & 0.1 & - \\
    Cutout~\cite{devries2017cutout}      & 0 & 0 & 16 & 0 & - \\
    Drop-Path Prob~\cite{larsson2016fractalnet}   & 0 & 0 & 0.2 & 0 & - \\
    BN calib batch size & 400 & 400 & 200 & 400 & - \\
    BN calib steps      & 25  & 25  & 100 & 25  & 0 \\
    \# GPUs       & 1 & 1 & 4 & 8 & 1 \\
    \hline
\end{tabular}
\end{table}

Basically, most of these settings are the same as the settings to train ground truth. A few notable adjustments include:

\begin{itemize}
    \item We manually tuned the learning rate used in NAS-Bench-101 and NAS-Bench-201 as we find the supernet hardly converging with large learning rate. Sometimes the training even blows up. Furthermore, we use SGD with gradient clip as optimizer.
    \item We manually tuned the batch size in DARTS-CIFAR10 and DARTS-PTB to better leverage the computation power of our hardware platform, so as to save the time for extended training.
    \item We adopt a \emph{multi-path parallel strategy} that samples different architectures on different GPUs every mini-batch. We then train these architectures with different data similar to data parallel. After backward propagation, gradients on all GPUs are averaged for updating. We find such parallelism is generally more scalable and can boost the supernet performance by up to 2\% (on DARTS-CIFAR10 and ProxylessNAS).
\end{itemize}

For ground truth training, we completely followed the settings mentioned in the original paper, unless otherwise specified. For DARTS-CIFAR10, we train on one GPU with batch size 96. For ProxylessNAS, we train on 8 GPUs with batch size 1024. We turned off batch-norm calibration during evaluation and used the batch-norm statistics calculated with momentum.

\subsection{Search Spaces}

Here is a detailed description of all the search spaces we have used, and how we have built the supernet to adopt weight sharing.

\subsubsection{NAS-Bench-101}

To make diagnose of one-shot methods possible and fully leverage previous-computed benchmark results, we design a sub search space of NAS-Bench-101~\cite{ying2019nasbench101}, which is also referred in NAS-Bench-1Shot1~\cite{zela2020nasbench1shot1}. Our search space is similar to search space 3 in NAS-Bench-1Shot1, with subtle differences to fully align with NAS-Bench-101:

\begin{itemize}
    \item We use the same channel number configuration as NAS-Bench-101.
    \item We force the number of intermediate nodes in a cell to be exactly 5, to avoid introducing an extra zero-op.
    \item In NAS-Bench-101, all intermediate nodes going to the output node of a cell, are concatenated, and then input node (after necessary 1x1 conv) is added to the output. This behavior makes constraining the number of parents of output not enough, as the channel number of intermediate nodes become output channel divided by the number of intermediate nodes (instead of all). To compensate this, we forbid the connection from input to output, force the output node to choose 2 from the intermediate 5.
    \item We do not deduplicate isomorphic cells.
\end{itemize}

In the end, we end up with 95985 different cells, and 42228 deduplicate isomorphic cells are counted. To train the supernet, we randomly sample one per mini-batch, from 95985, and update the corresponding weights. We kept a fixed set of 1k architectures out of 95985 for evaluating, which has the distribution shown in \autoref{fig:efficiency-performance-nb101}.

Following the guidelines recommended by NAS-Bench-101, we split the original CIFAR-10 training data into a training set consisting of 40k images and a validation set consisting of 10k images. We use the training set of supernet training, validation set for model selection, i.e., to evaluate architectures on supernet and choose the best architecture, while the original test set is used to evaluate the one single test model chosen. Supernet training takes about 1 day every 2k epochs on a single V100 GPU.

\begin{figure}
    \centering
    \begin{subfigure}{.48\textwidth}
        \centering
        \includegraphics[width=\textwidth]{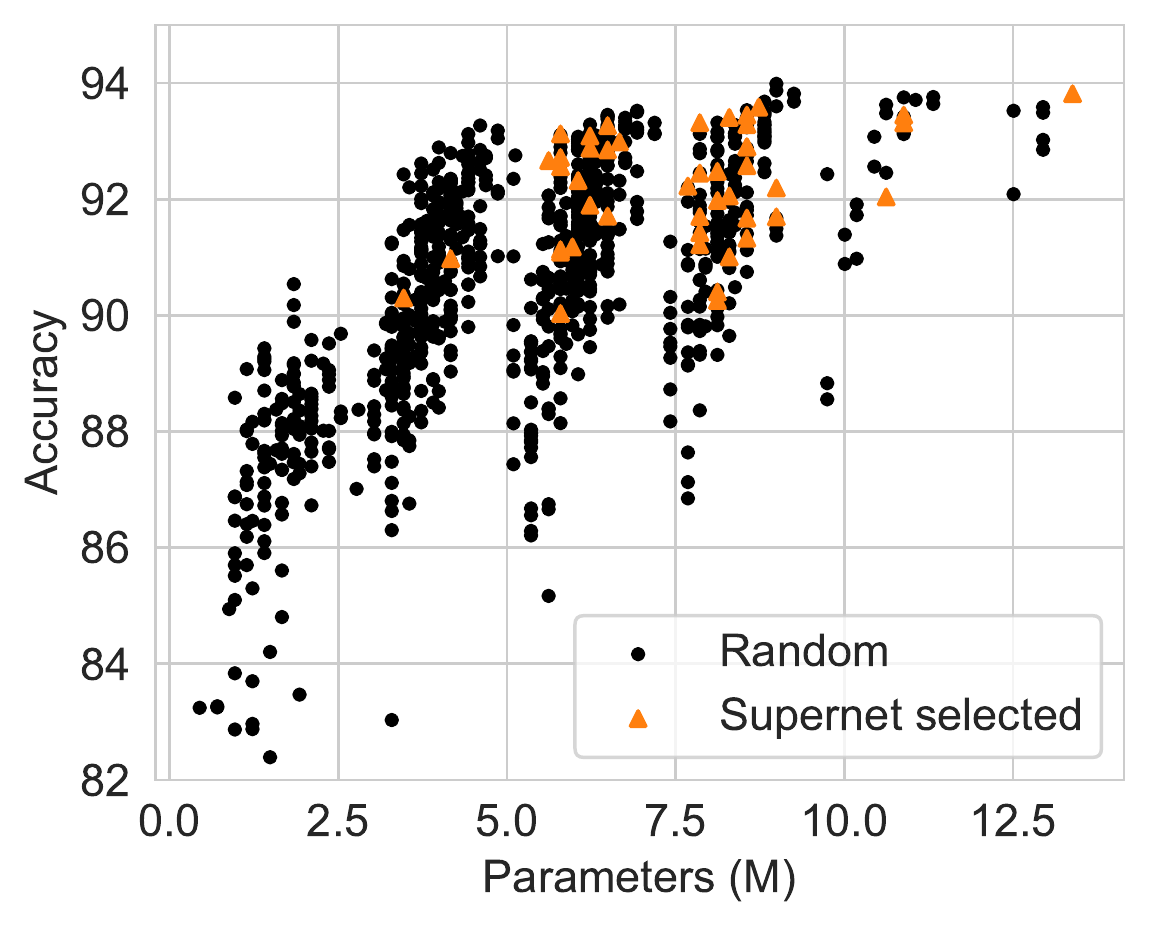}
        \caption{NAS-Bench-101}
        \label{fig:efficiency-performance-nb101}
    \end{subfigure}
    \begin{subfigure}{.48\textwidth}
        \centering
        \includegraphics[width=\textwidth]{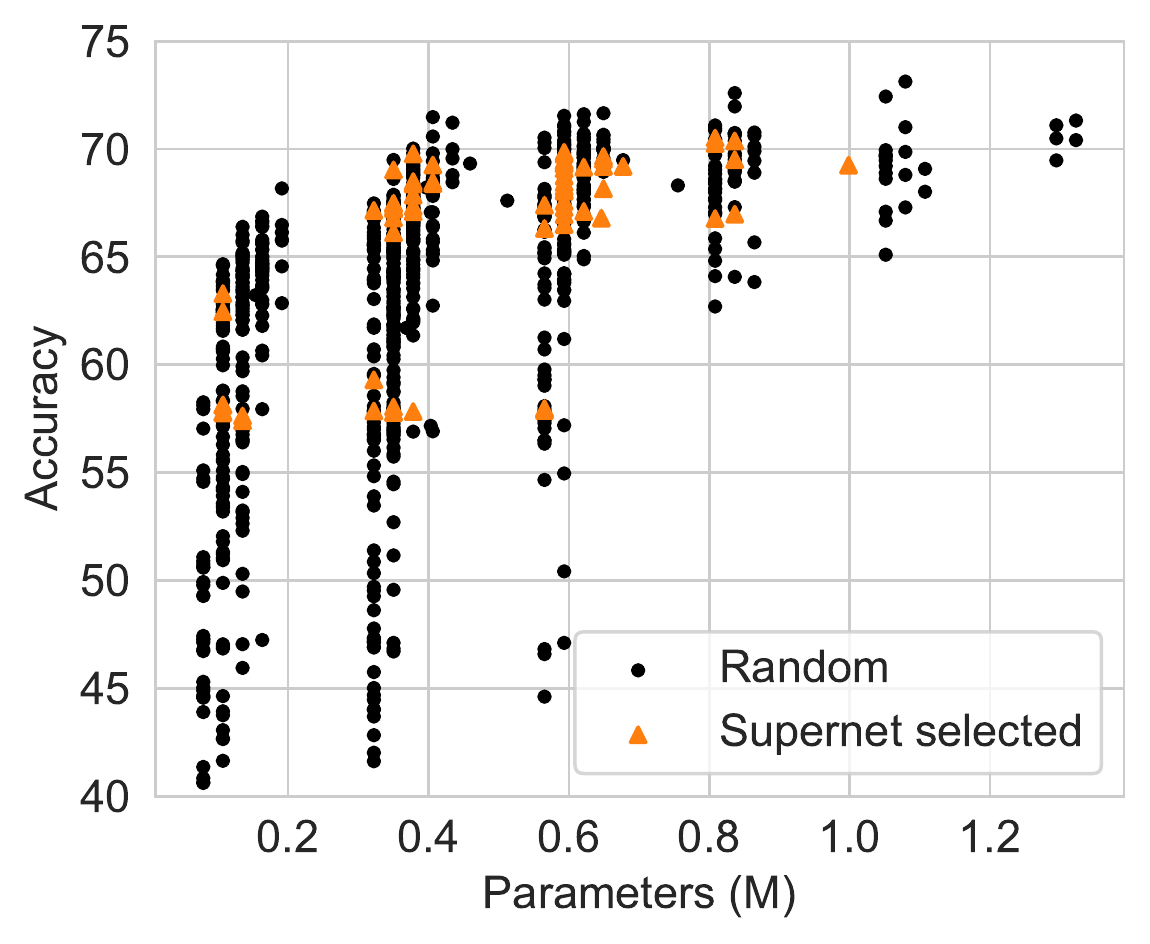}
        \caption{NAS-Bench-201}
        \label{fig:efficiency-performance-nb201}
    \end{subfigure}
    \caption{Distributions of parameters and test accuracy of 1k candidate models on NAS-Bench-101 and NAS-Bench-201. We use orange for architectures chosen at least once by any naively trained supernet, i.e., supernets trained simply with various epochs. We use black for others.}
\end{figure}

\subsubsection{NAS-Bench-201}

NAS-Bench-201~\cite{dong2020nasbench201} constructs its cell with 4 nodes connected with 6 edges, with an operator choosing from 5 candidate operators on each edge. As it is designed for one-shot NAS, almost no change is needed to apply supernet training. However, in NAS-Bench-201 there are some invalid cells, where input node of the cell is completely not connected to output node, and they cannot be trained at all. We devise a filter to avoid those invalid cells from being chosen. In fact, only 341 cells are invalid, and 15284 out of 15625 are kept. Similar to NAS-Bench-101, we kept a fixed set of 1k architectures out of 15284 for evaluating, which has the distribution shown in \autoref{fig:efficiency-performance-nb201}.

Though the original NAS-Bench-201 is given across three different scaled image classification datasets, we use CIFAR-100 only as the other two have been experimented on other search spaces. Supernets of NAS-Bench-201 are trained on NAS-Bench-201 unless otherwise specified. Following the authors' practice, we use the original training set for supernet training, and original validation set for both validation and final model testing. Training of 4k epochs takes 35 hours on a single V100 GPU.

\subsubsection{DARTS-CIFAR10}

The CIFAR10 search space adopted in DARTS~\cite{liu2018darts} is very similar to the ones used in \cite{pham2018efficient,zoph2018learning}, except that all nodes in a cell are concatenated into the output and there are subtle differences in convolution with stride = 2 in reduction cell. Since we are not using gradient-based methods, instead of building a supernet with all combinations of input choices and operator choices expanded, like \cite{liu2018darts}, we follow the practice of ENAS~\cite{pham2018efficient} by creating only two choice blocks for each node, so that a single choice block can be shared even if its input node varies. However in DARTS, the stride of convolution in reduction cell depends on which input it has chosen. Luckily, changing the stride of a convolution has no effect on its parameters. Therefore we determine the stride of convolution dynamically during training time when a particular architecture has been chosen. The channels and number of cells are kept exactly consistent between search phase and architecture evaluation phase. It takes about 1 day on 4 V100 GPUs to train the supernet for 1k epochs.

To align with the ground truth training used in DARTS, we use the original training set (50k images) for both supernet and ground truth training, and the original validation set for validation, architecture selection and testing. Standalone training of one model takes about 30 to 50 hours on one V100 GPU, depending on the model size. Altogether, we have trained 377 architectures from scratch, for which we show their distribution in \autoref{fig:efficiency-performance-darts}.

\begin{figure}
    \centering
    \begin{subfigure}{.48\textwidth}
        \centering
        \includegraphics[width=\textwidth]{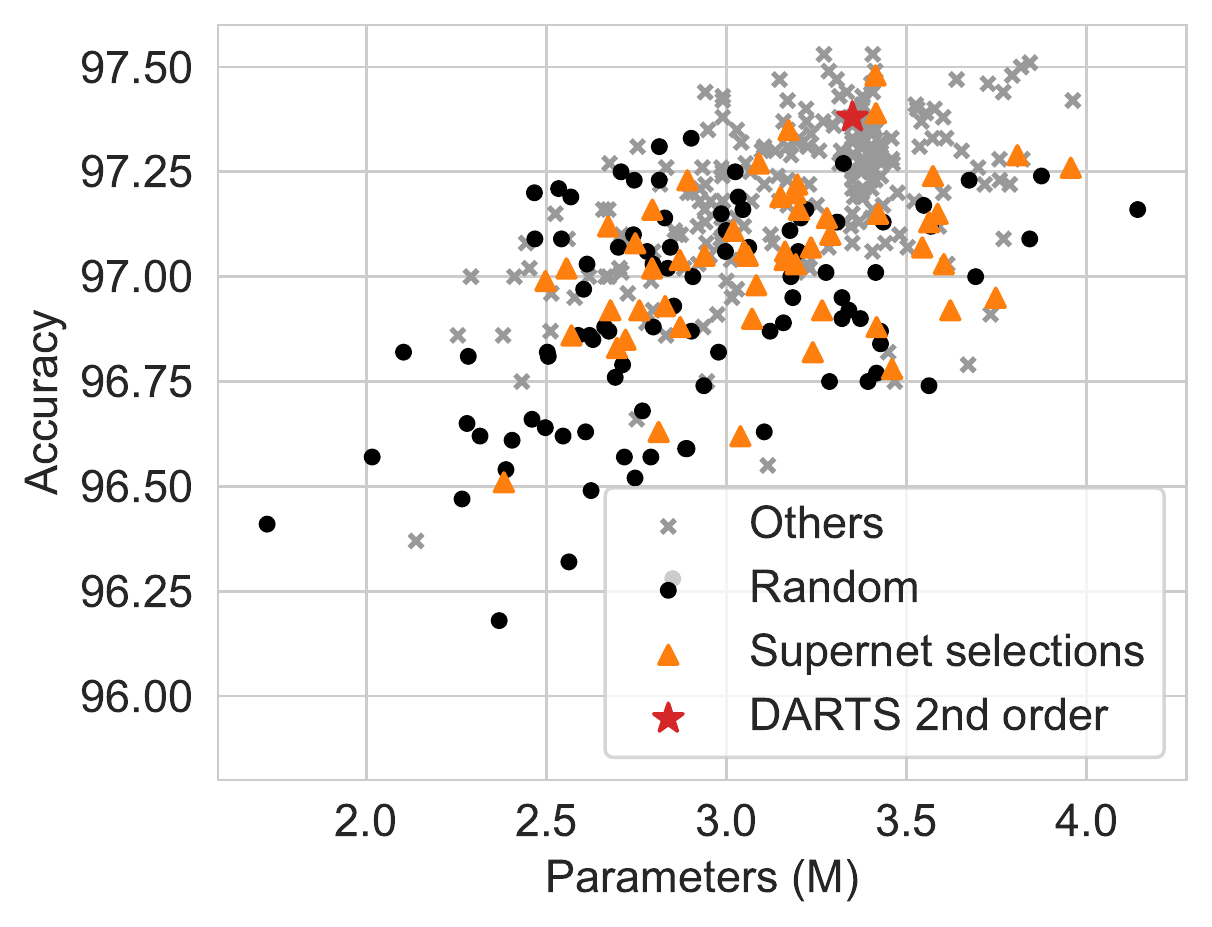}
    \end{subfigure}
    \begin{subfigure}{.48\textwidth}
        \centering
        \includegraphics[width=\textwidth]{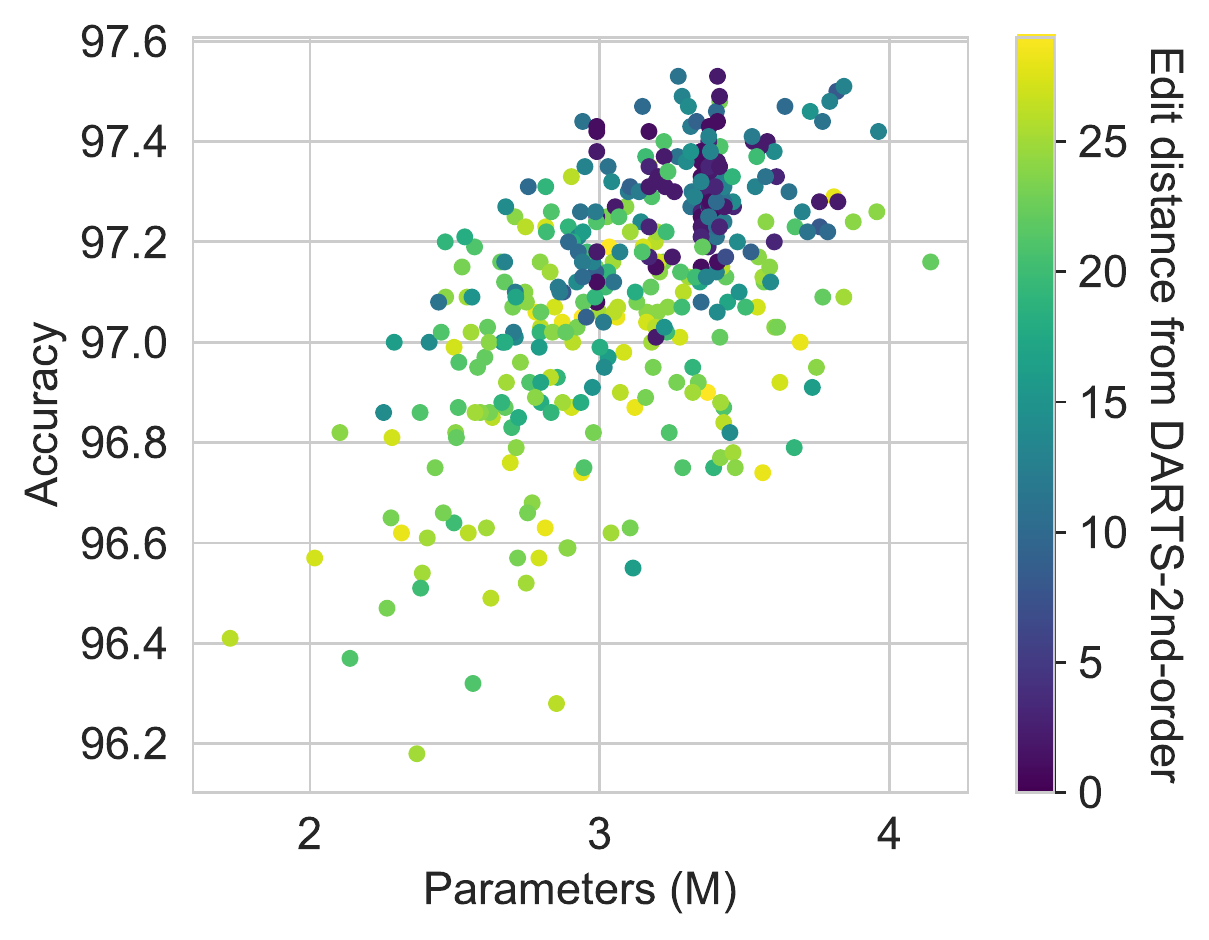}
    \end{subfigure}
    \caption{Distributions of parameters and validation accuracy of 377 architectures on DARTS-CIFAR10. We use orange for architectures chosen at least once by any naively trained supernet, black for a randomly chosen subset architectures of size 100, grey for others. DARTS (second order), which is the architecture reported in the original paper, is marked with star. In figure right, we compare each architecture in the chart with the architecture reported in DARTS, and report their edit distance. Notably, most of the architectures with small edit distances are selected in the pruning experiments.}
    \label{fig:efficiency-performance-darts}
\end{figure}

\subsubsection{ProxylessNAS}

Following ProxylessNAS~\cite{cai2018proxylessnas}, we use the space in its GPU setting. Concretely, it is built upon MobileNetV2~\cite{sandler2018mobilenetv2} and allowing most of mobile inverted convolution layers to choose from kernel size $\{3, 5, 7\}$ and expansion ratios $\{3, 6\}$. For those choice blocks that do not change the input tensor shape, ProxylessNAS further allows them to be skipped. As ProxylessNAS-GPU is using width multiplier 1.35, we followed such setting and width multiplier is directly applied starting from supernet training. When training, all the architectures are equally likely to be sampled. In evaluation, we consider two settings in this paper. Proxyless-600M is to filter the architectures with FLOPs greater than 600M (only the models that fit mobile settings will be evaluated). If this is not specified, we simply consider all the possible architectures as legal.

To make the supernet performance directly comparable to ground truth performance, we also use the original training set (1.28M images) as training set, and the held-out validation set of 50k images for validation and testing. It takes about 7 days to train a supernet with 1k epochs on 8 V100 GPUs, while training a single model takes 35 hours on 8 V100 GPUs. Altogether we have trained 36 models from scratch, the distribution of which is shown in \autoref{fig:efficiency-performance-proxyless}.

\begin{figure}
    \centering
    \begin{subfigure}{.48\textwidth}
        \centering
        \includegraphics[width=\textwidth]{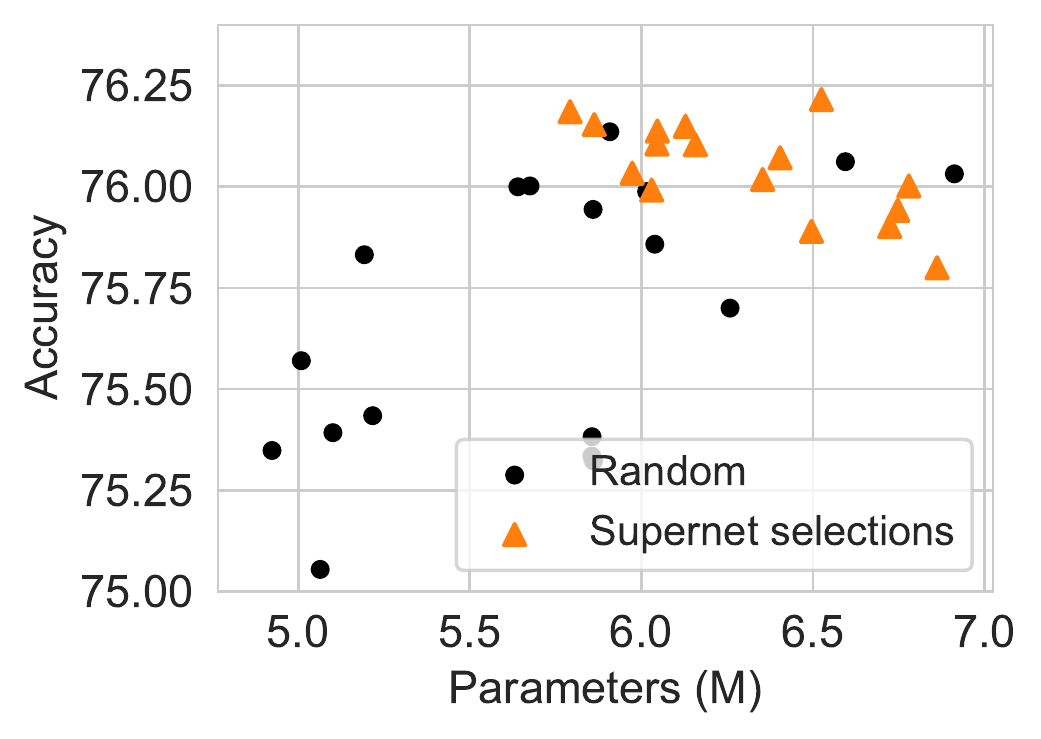}
    \end{subfigure}
    \begin{subfigure}{.48\textwidth}
        \centering
        \includegraphics[width=\textwidth]{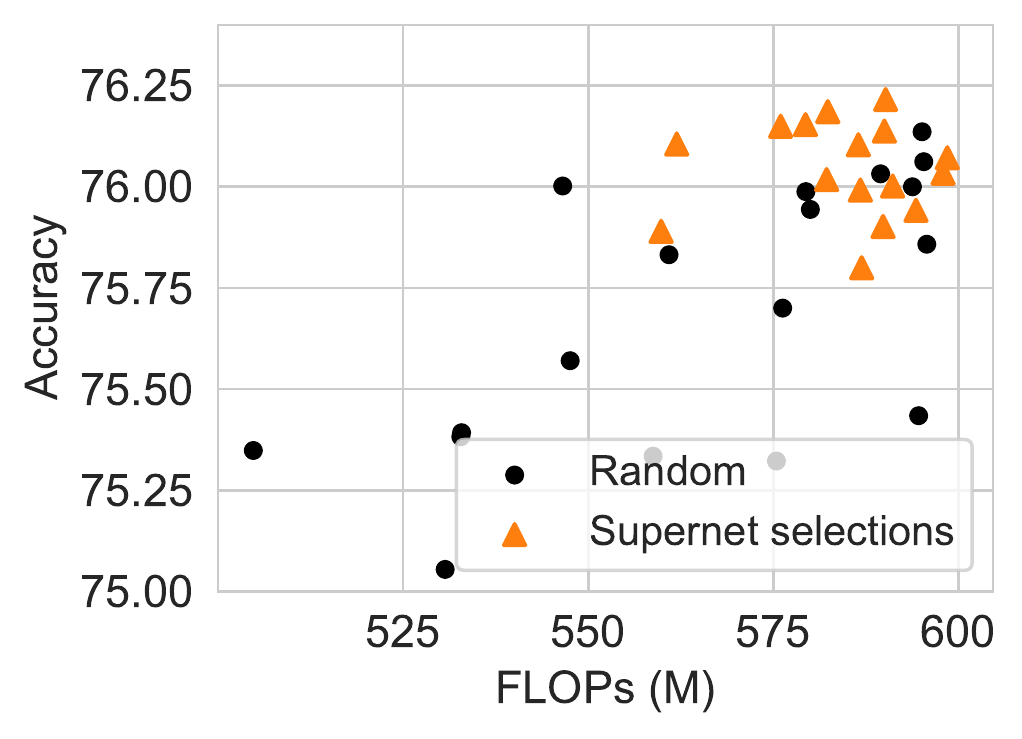}
    \end{subfigure}
    \caption{Distributions of parameters, FLOPs and validation accuracy of 36 architectures on ProxylessNAS. We use orange for architectures chosen at least once by any naively trained supernet, black for a randomly chosen subset architectures.}
    \label{fig:efficiency-performance-proxyless}
\end{figure}

\subsubsection{DARTS-PTB}

The architecture space searches for an RNN cell, consisting of 8 hidden states, each of which picks an activation function out of 4 and its input from its predecessors. We exactly follow the standalone training settings used in \cite{liu2018darts} for supernet training, which means, we kept channels unchanged, did not add batch normalization after each hidden state, and used the exactly same ASGD/SGD switching rule to train the supernet instead of Adam optimizer.

Since Penn Treebank has an official train, valid and test split, we use the validation set to determine when to change the type of optimizer and guide the model selection. After that, test set is used to do the final evaluation. We use batch size = 1 on test set, but batch size = 10 on validation set to accelerate evaluation.

\begin{figure}
    \centering
    \begin{subfigure}{.48\textwidth}
        \centering
        \includegraphics[width=\textwidth]{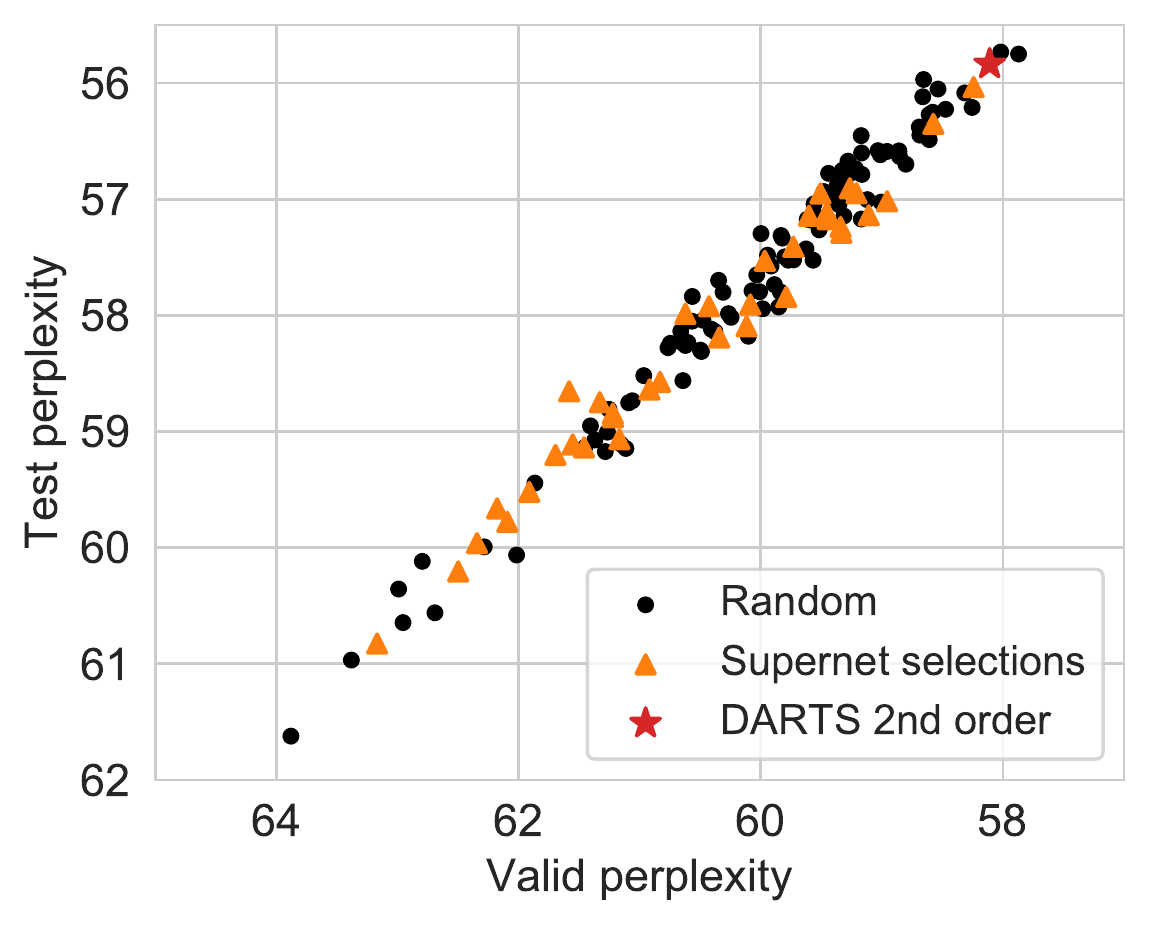}
        \caption{Validation}
    \end{subfigure}
    \begin{subfigure}{.48\textwidth}
        \centering
        \includegraphics[width=\textwidth]{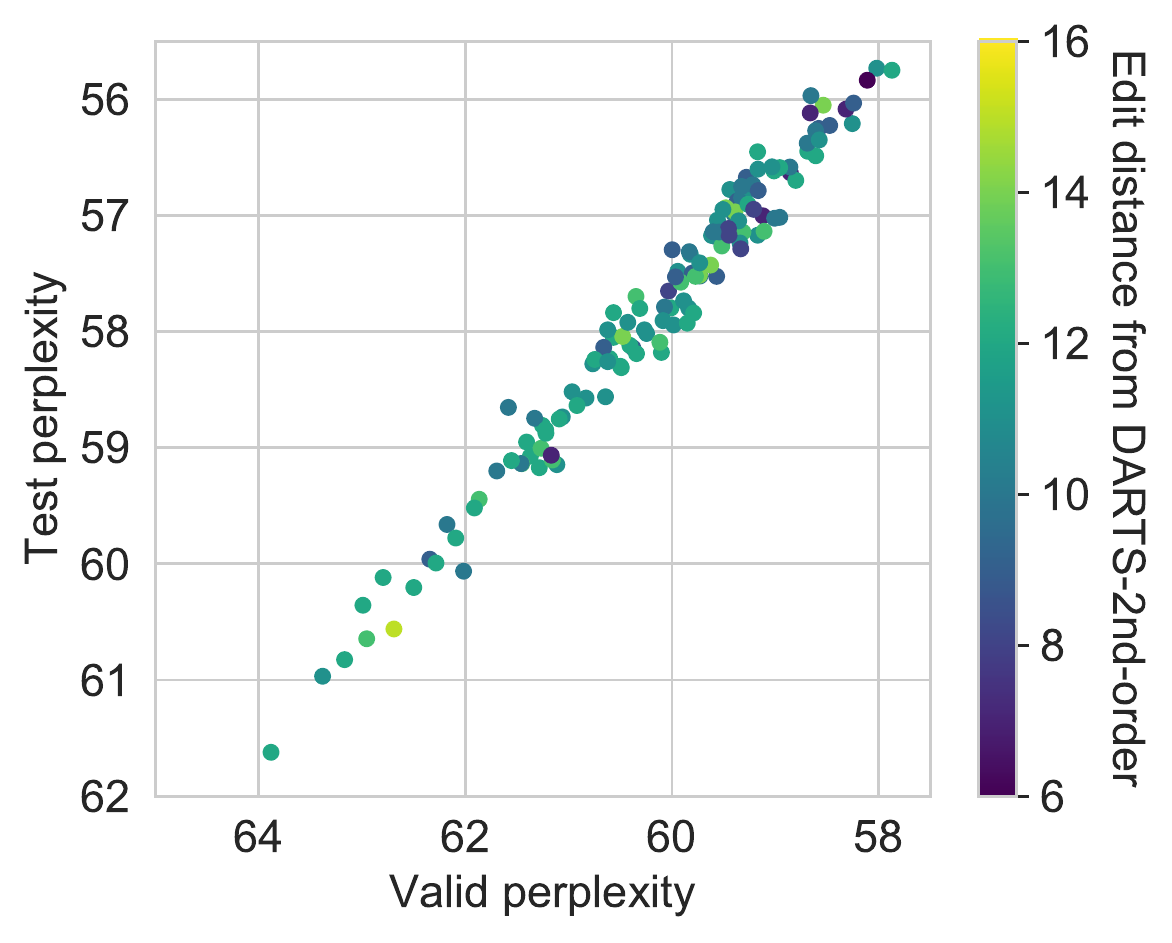}
        \caption{Compared to edit distance}
    \end{subfigure}
    \caption{Distributions of validation and test perplexity of 137 architectures on DARTS-PTB. We use orange for architectures chosen at least once by any naively trained supernet, black for a randomly chosen subset architectures of size 100, grey for others. DARTS (second order), which is the architecture reported in the original paper, is marked with star. Similar to \autoref{fig:efficiency-performance-darts}, we also show the edit distance for each architecture.}
    \label{fig:efficiency-performance-ptb}
\end{figure}

\section{Stability and Reproducibility}

\subsection{Exploring Supernet Training Tricks}

Note that most of the experiments in this paper are run with a pre-defined training approach. For example, the supernets are trained with a pre-defined learning rate, batch size and etc. With the naive single-path training as baseline, we adopt several possible variations, including: altering learning rate and weight decay, initializing with a different seed, multi-path training that feeds the same data into multiple architecture and aggregates the gradient to update~\cite{yang2019cars,pham2018efficient,you2020greedynas} and FairNAS~\cite{chu2019fairnas}. For a fair comparison under the same budget, for multi-path and FairNAS we only use one third of the original epochs as for each mini-batch (one fifth for NAS-Bench-201), three architectures are sampled and trained (five for NAS-Bench-201). Results are shown in \autoref{tab:supernetstab}.

\begin{table}[htbp]
    \centering
    \caption{Comparison of correlation with ground truth (Corr-GT), supernet-top-10 ground truth (Top-10), supernet performance (S-Perf) and correlation with baseline (Corr-BL) under different supernet training settings.}
    \label{tab:supernetstab}
    \begin{tabular}{c|c|c|c|c}
    \hline
                              Group & Corr-BL & Corr-GT $\uparrow$ ($\Delta$) & Top-10 $\uparrow$ ($\Delta$) & S-Perf $\uparrow$ ($\Delta$) \\
    \hline
    NAS-Bench-101 (1k epochs)       &   1.000 &                0.618 &                93.45 &                88.38 \\
    FairNAS~\cite{chu2019fairnas}   &   0.967 &  0.683 (\textcolor{blue}{+0.064}) &  93.64 (\textcolor{blue}{+0.19}) &   86.59 (\textcolor{red}{-1.79}) \\
    Multi-Path~\cite{pham2018efficient} &   0.963 &  0.626 (\textcolor{blue}{+0.007}) &  93.87 (\textcolor{blue}{+0.42}) &   85.99 (\textcolor{red}{-2.38}) \\
    LR=0.05, WD=$3 \cdot 10^4$      &   0.982 &   0.608 (\textcolor{red}{-0.010}) &   93.13 (\textcolor{red}{-0.32}) &  88.86 (\textcolor{blue}{+0.49}) \\
    Different Seed                  &   0.982 &  0.630 (\textcolor{blue}{+0.012}) &  93.59 (\textcolor{blue}{+0.14}) &   87.57 (\textcolor{red}{-0.80}) \\
    \hline
    NAS-Bench-101 (2k epochs)       &   1.000 &                0.659 &                93.82 &                90.58 \\
    FairNAS                         &   0.964 &   0.652 (\textcolor{red}{-0.007}) &   93.41 (\textcolor{red}{-0.41}) &   90.32 (\textcolor{red}{-0.26}) \\
    Multi-Path                      &   0.963 &   0.656 (\textcolor{red}{-0.002}) &   93.64 (\textcolor{red}{-0.18}) &   90.29 (\textcolor{red}{-0.29}) \\
    LR=0.05, WD=$3 \cdot 10^4$      &   0.970 &   0.611 (\textcolor{red}{-0.048}) &   93.45 (\textcolor{red}{-0.37}) &  90.58 (\textcolor{blue}{+0.01}) \\
    Different Seed                  &   0.979 &   0.644 (\textcolor{red}{-0.014}) &   93.45 (\textcolor{red}{-0.37}) &   90.29 (\textcolor{red}{-0.28}) \\
    \hline
    NAS-Bench-201 (2k epochs)       &   1.000 &                0.701 &                  69.66 &                  49.01 \\
    FairNAS &   0.978 &  0.716 (\textcolor{blue}{+0.015}) &  69.87 (\textcolor{blue}{+0.21}) &    48.74 (\textcolor{red}{-0.27}) \\
    Multi-Path &   0.984 &  0.706 (\textcolor{blue}{+0.005}) &  70.05 (\textcolor{blue}{+0.39}) &    48.73 (\textcolor{red}{-0.28}) \\
    CIFAR-10 &   0.915 &  0.831 (\textcolor{blue}{+0.130}) &  69.87 (\textcolor{blue}{+0.21}) &  81.95 (\textcolor{blue}{+32.94}) \\
    ImageNet-16-120 &   0.962 &  0.711 (\textcolor{blue}{+0.010}) &  69.72 (\textcolor{blue}{+0.06}) &   21.81 (\textcolor{red}{-27.20}) \\
    \hline
\end{tabular}

\end{table}

Empirically we find no significant changes in the numbers we reported. Tricks like Multi-Path and FairNAS show an advantage in finding better models at 1k epochs, but little improvement at 2k. Sometimes applying tricks might even harm the supernet performance, compared to baseline. Despite all subtle differences, the rank correlation with respect to baseline is always high (above 0.95), which means that the rank of supernet is stable across all attempted setups --- all these supernets end up with a similar bias.

Refer to \autoref{fig:all-correlation-nb101}, \autoref{fig:all-correlation-nb201} and \autoref{fig:all-correlation-others} for the mutual correlations among all trained supernets and ground truths.

\subsection{Robustness of Ground Truth}

Though authors of NAS-Bench-101 and NAS-Bench-201 both reported that their architecture rank is relatively stable when different random seed is used (spearman correlation above 0.95 for NAS-Bench-101 and 0.98 for NAS-Bench-201), we find that this is not the case of DARTS-CIFAR10 and DARTS-PTB. As we retrain 100 architectures with a different seed, the rank becomes relatively unstable, as shown in \autoref{fig:stability-darts-ptb}. Such instability comes not as a surprise to us because it has been already observed in \cite{liu2017hierarchical,liu2018darts,yang2019nas} that performance on CIFAR-10 has high variance even with an exactly same setup.

\begin{figure}
    \centering
    \begin{subfigure}{.35\textwidth}
        \centering
        \includegraphics[width=\textwidth]{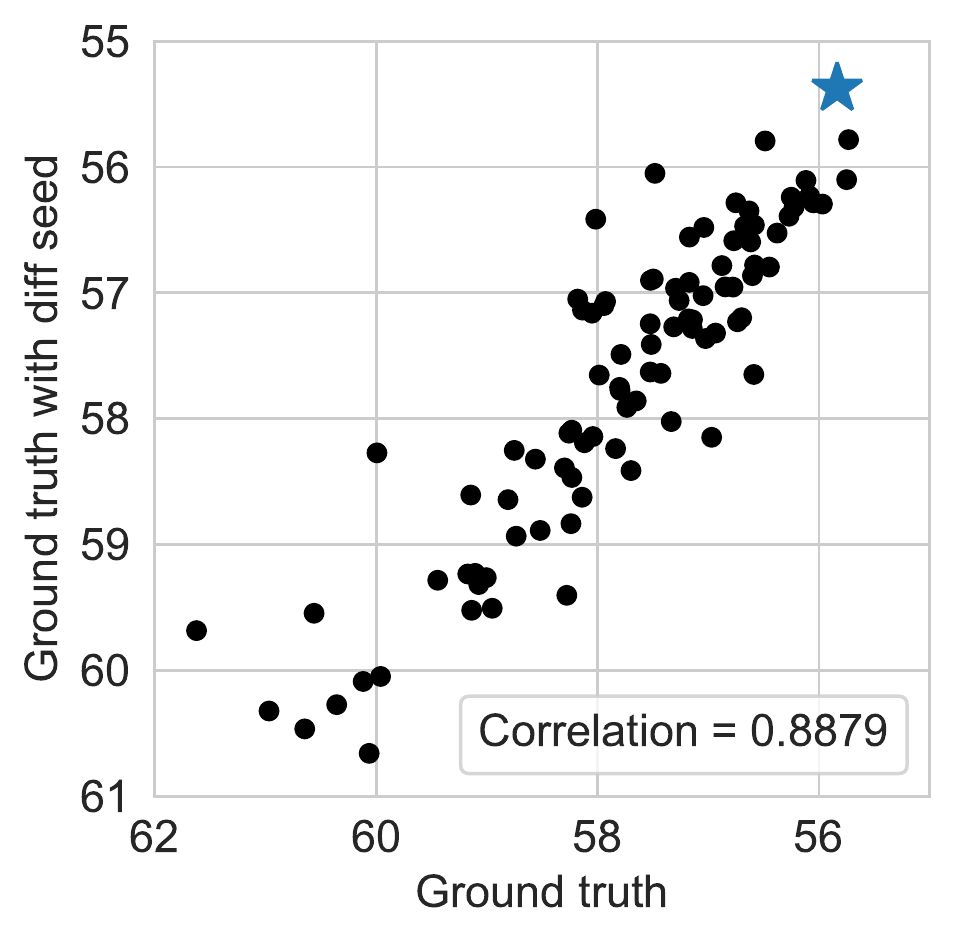}
        \caption{DARTS-PTB}
    \end{subfigure}
    \begin{subfigure}{.48\textwidth}
        \centering
        \includegraphics[width=\textwidth]{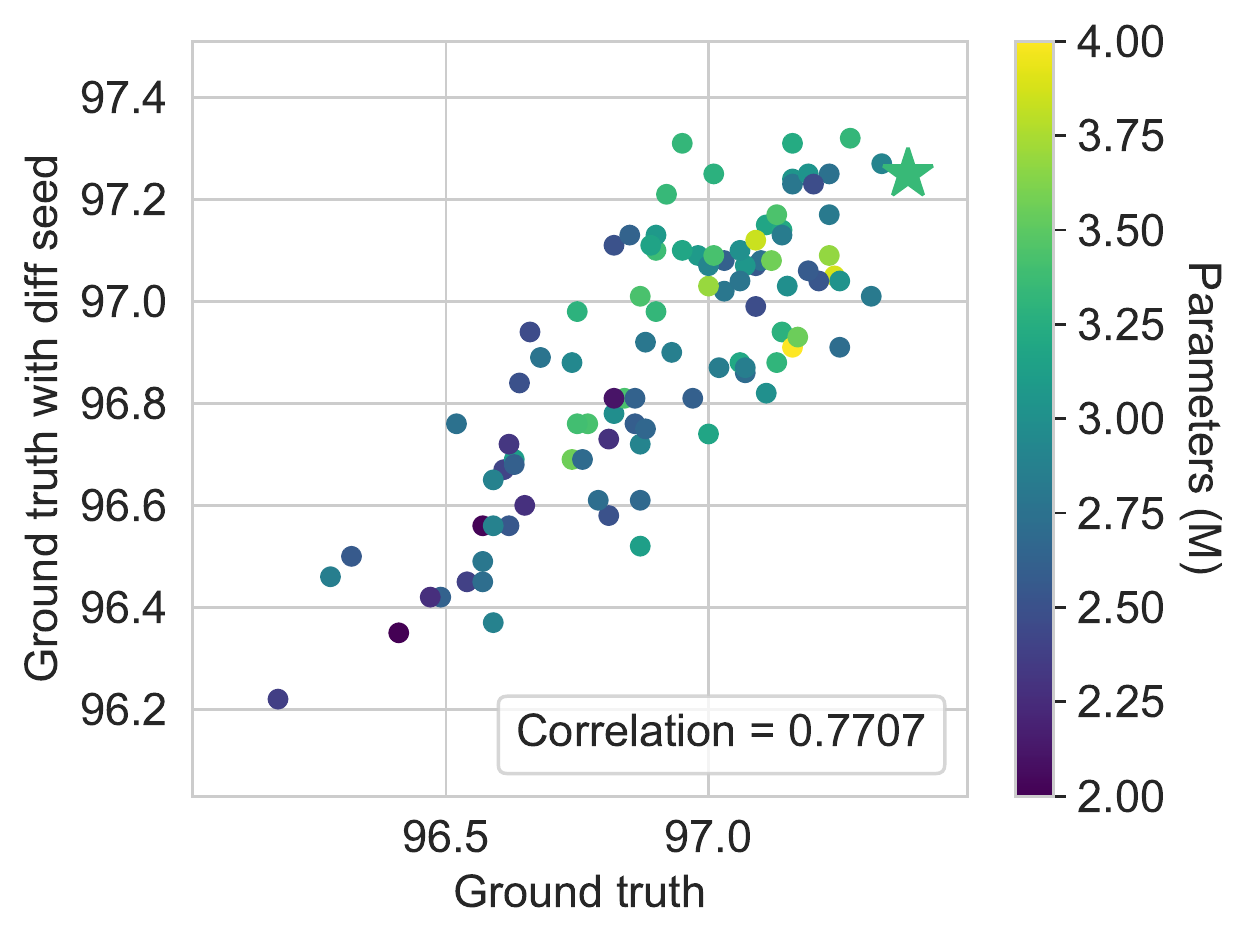}
        \caption{DARTS-CIFAR10}
    \end{subfigure}
    \caption{Stability of architecture rank subject to different random seeds. Similar to \autoref{fig:efficiency-performance-darts} and \autoref{fig:efficiency-performance-ptb}, we mark the architecture found by DARTS with star.}
    \label{fig:stability-darts-ptb}
\end{figure}

On NAS-Bench-101 and NAS-Bench-201, we verified that training with seed does not have a large effect on architecture rank. However, if we purposely use a very different training approach, the architecture rank still varies. For example, on NAS-Bench-101, inspired by the hyper-parameter setup used in ENAS~\cite{pham2018efficient}, DARTS~\cite{liu2018darts} and some follow-up works~\cite{yang2019nas}, we change the number of epochs to 540, which is 5$\times$ of the epochs used in original paper. optimizer to SGD with momentum 0.9, gradient clipping to 5. We use Drop-Path~\cite{larsson2016fractalnet} with probability 0.1, Cutout~\cite{devries2017cutout} with length 16, auxiliary head~\cite{szegedy2015googlenet} with weight 0.4. On NAS-Bench-201, we increase the initial convolution filters to 128, cutout to 16, gradient clipping to 5 and epochs to 600. Results are shown in \autoref{fig:stability-nasbench-augment}.

\begin{figure}
    \centering
    \begin{subfigure}{.4\textwidth}
        \centering
        \includegraphics[width=\textwidth]{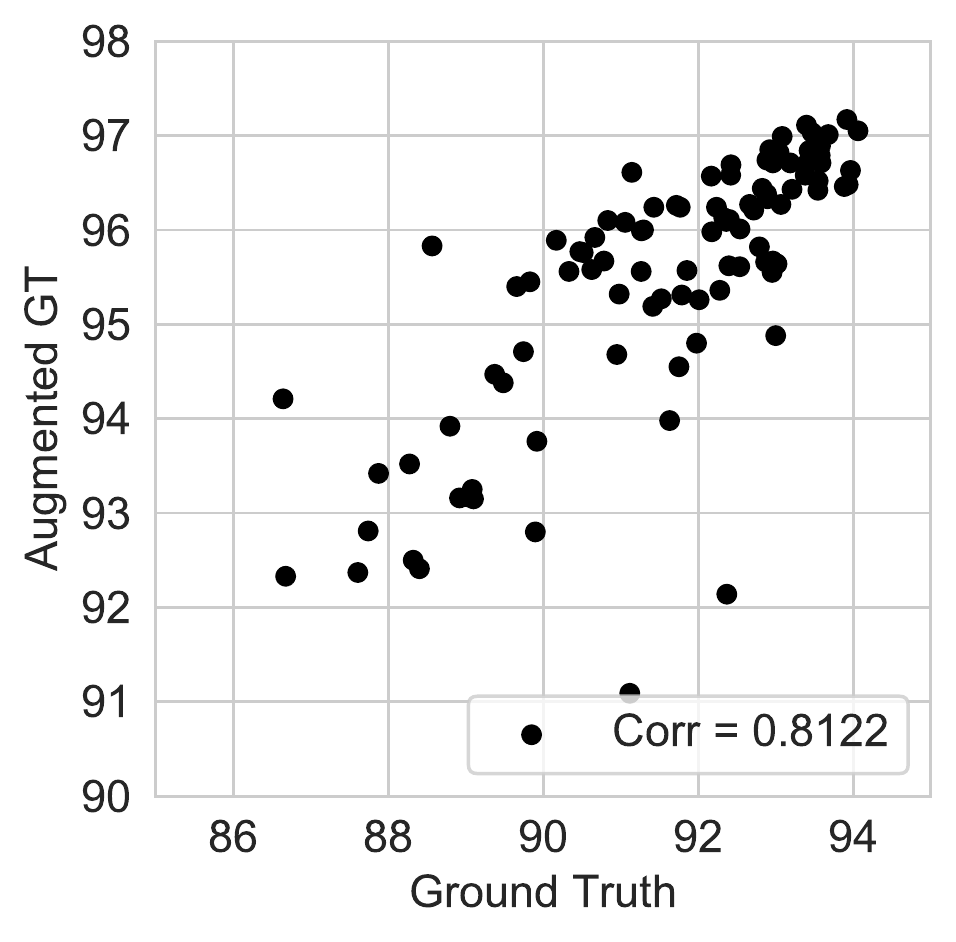}
        \caption{NAS-Bench-101}
    \end{subfigure}
    \begin{subfigure}{.4\textwidth}
        \centering
        \includegraphics[width=\textwidth]{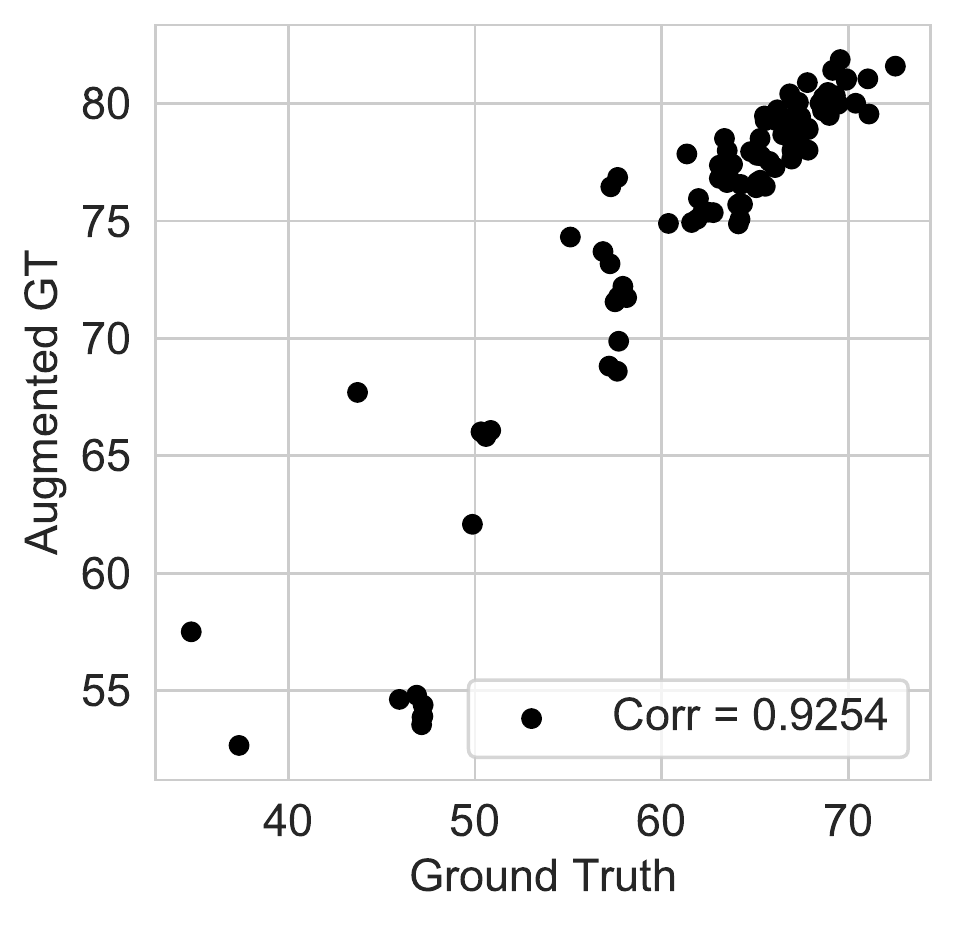}
        \caption{NAS-Bench-201}
    \end{subfigure}
    \caption{Stability of architecture rank subject to different training approaches.}
    \label{fig:stability-nasbench-augment}
\end{figure}

Despite that such instability exists, there is still a clear trend that some good architectures perform consistently well. Top-1 architecture under one setup might be not the best in another, but still very close in its absolute value. Nevertheless, to clarify, in this paper, when we refer to ground truth, we mean the stand-alone performance trained with a particular setup, and a particular random seed if necessary. 

\section{Omitted Tables and Figures}

Below we show the omitted tables and figures.

\begin{table}[htbp]
    \centering
    \caption{The performance of our best-trained supernet on different search spaces. For budgets, we compute the relative value with respect to the number of epochs to train a single architecture, i.e., ground truth. We reported the average, best, worst and difference between best and worst performance on sampled architectures, and similarly for ground truth.}
    \label{tab:performance1}
    \begin{tabular}{c|c|cccc|cccc}
    \hline
    & & \multicolumn{4}{c|}{Supernet} & \multicolumn{4}{c}{Ground Truth} \\ \cline{3-10}
    Search Space &        Budgets &   Avg &  Best &  Worst & Range &   Avg &  Best &  Worst & Range \\
    \hline
    NB-101 &  148.1$\times$ & 91.21 & 94.22 &  64.51 & 29.71 & 90.71 & 94.53 &  34.38 & 60.16 \\
    NB-201 &   20.0$\times$ & 50.90 & 64.86 &  19.78 & 45.08 & 62.74 & 73.13 &   9.77 & 63.36 \\
     DARTS &   13.3$\times$ & 92.87 & 94.57 &  82.72 & 11.85 & 96.91 & 97.38 &  96.18 &  1.20 \\
 Proxyless &    3.3$\times$ & 73.26 & 74.90 &  67.74 &  7.15 & - &     - &      - &     - \\
       PTB &    1.3$\times$ & 66.31 &  64.75 & 71.57 & 6.81 & 60.04 & 57.87 &  63.88 &  6.01 \\
    \hline
\end{tabular}

\end{table}

\begin{figure}[htbp]
    \centering
    \includegraphics[width=\textwidth]{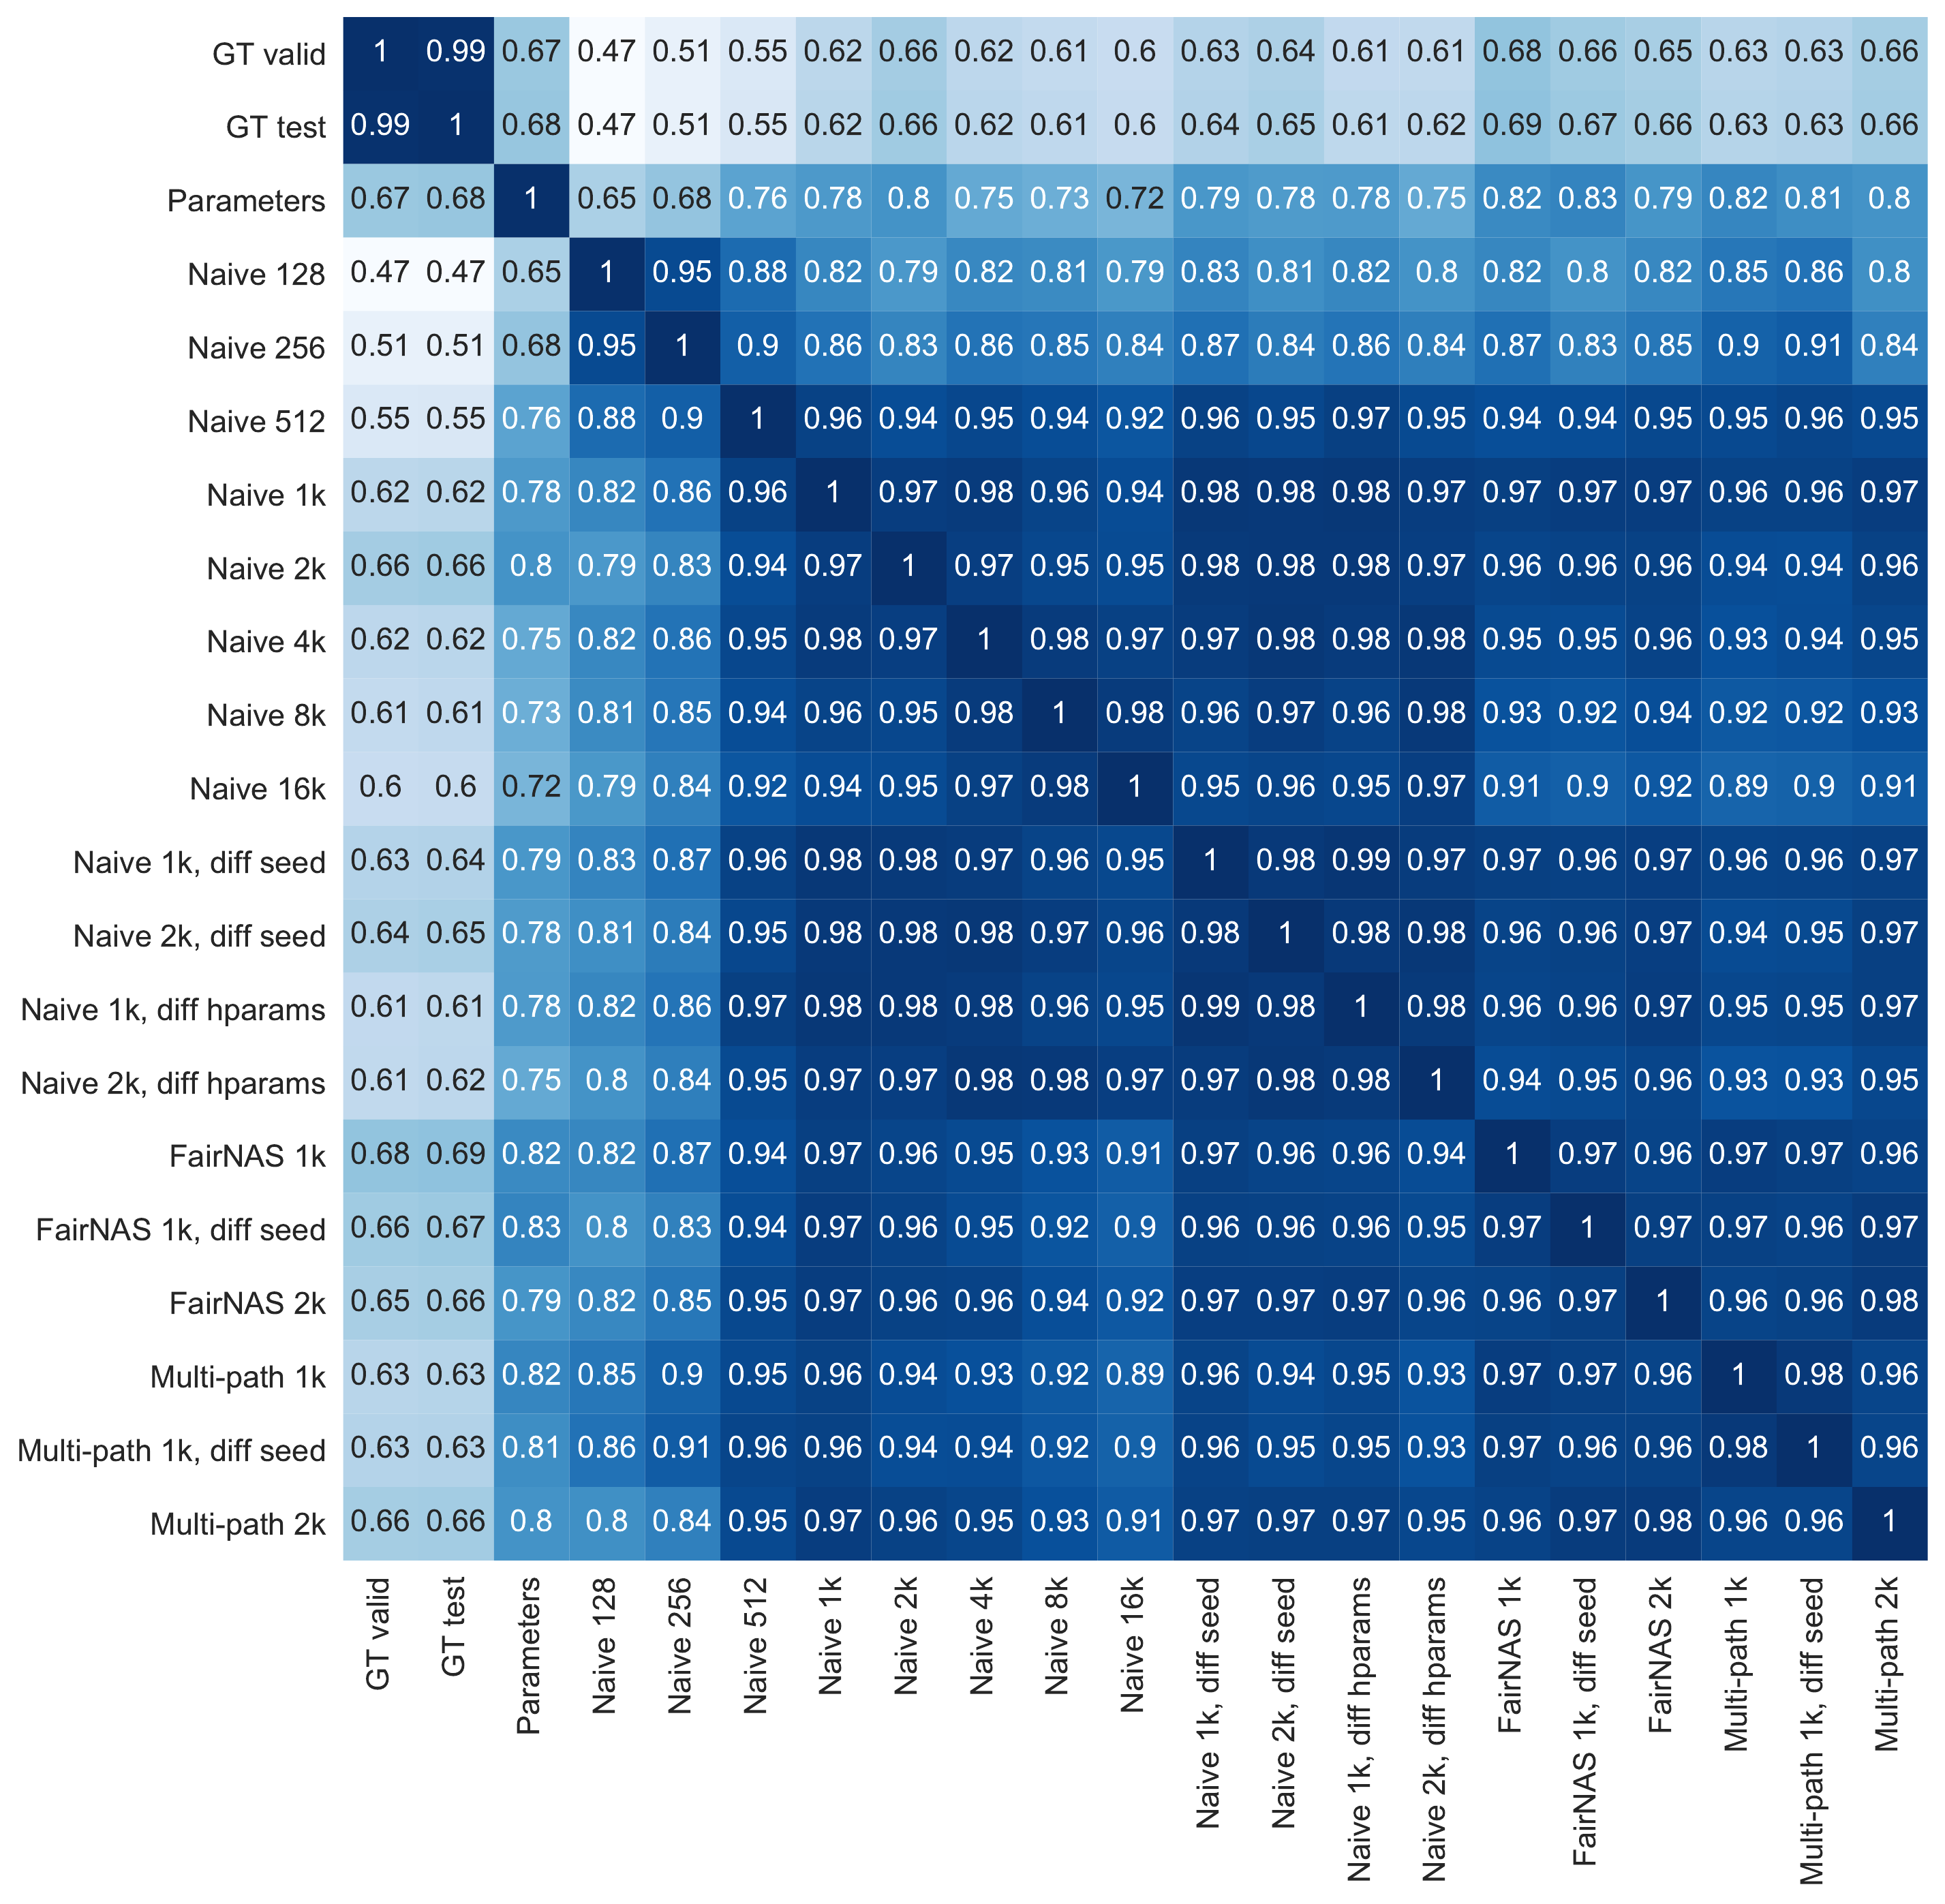}
    \caption{Mutual correlations of all trained supernets and ground truths on NAS-Bench-101}
    \label{fig:all-correlation-nb101}
\end{figure}

\begin{figure}[htbp]
    \centering
    \includegraphics[width=\textwidth]{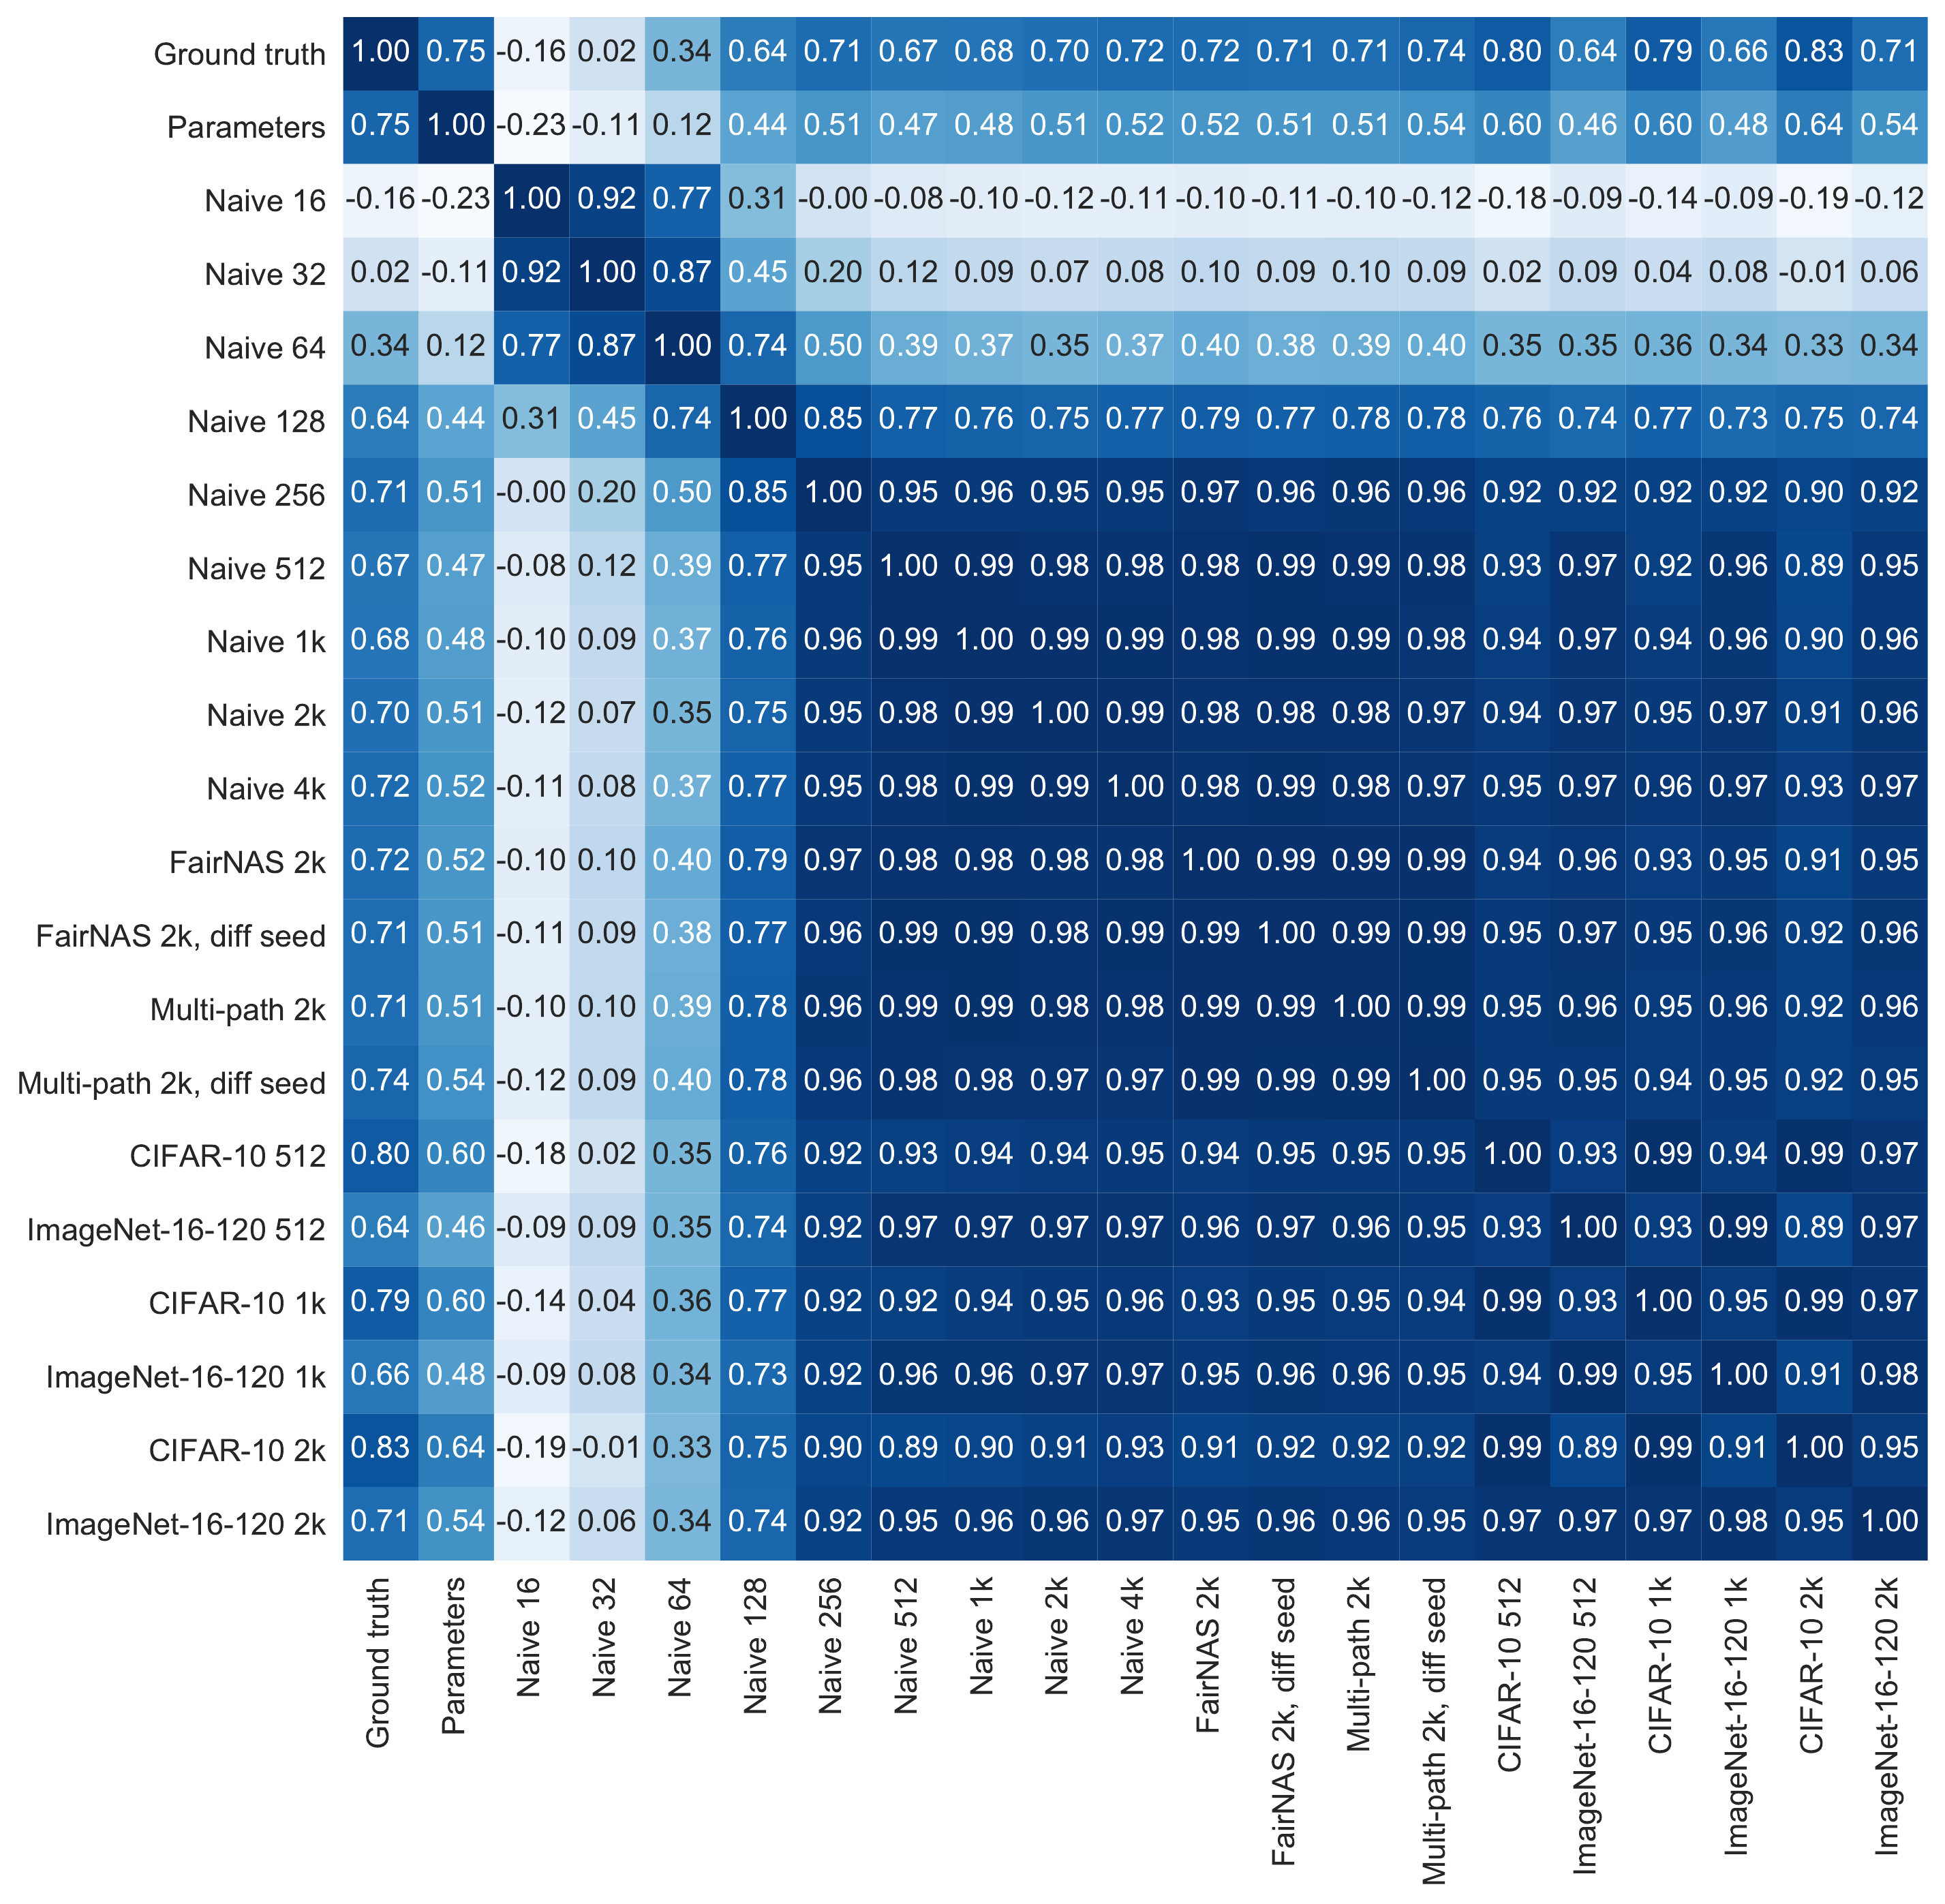}
    \caption{Mutual correlations of all trained supernets and ground truths on NAS-Bench-201}
    \label{fig:all-correlation-nb201}
\end{figure}

\begin{figure}[htbp]
    \centering
    \begin{subfigure}{.48\textwidth}
        \centering
        \includegraphics[width=\textwidth]{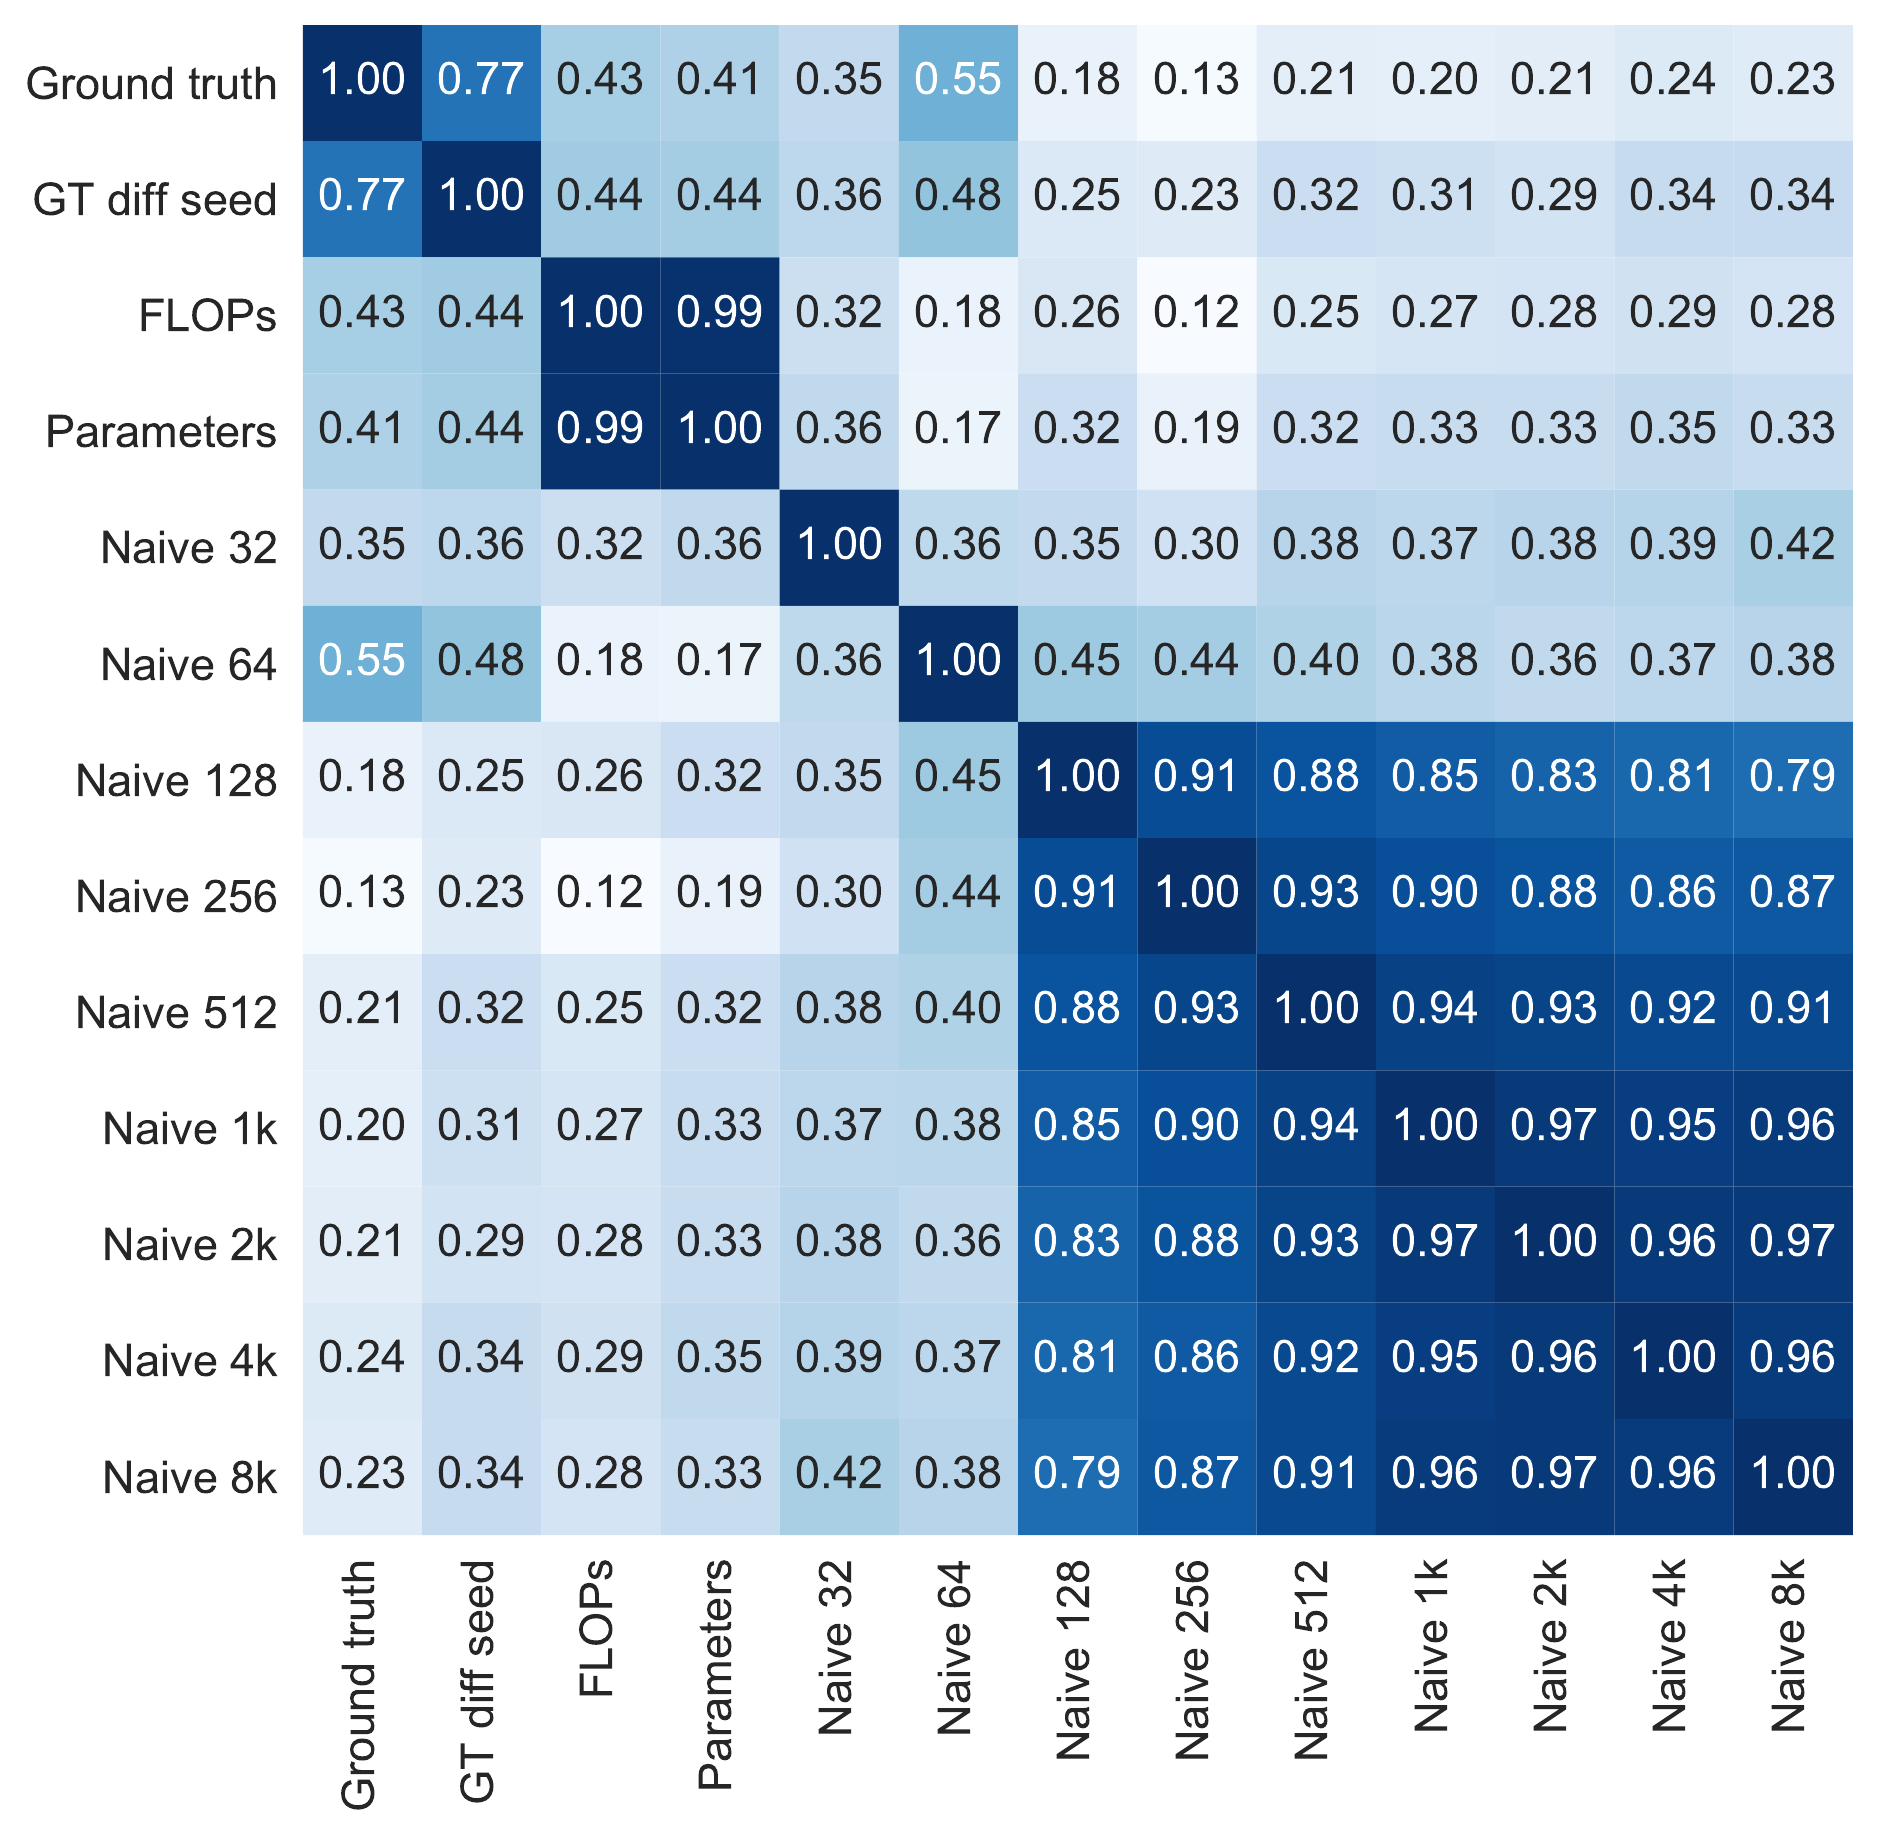}
        \caption{DARTS-CIFAR10}
    \end{subfigure}
    \begin{subfigure}{.48\textwidth}
        \centering
        \includegraphics[width=\textwidth]{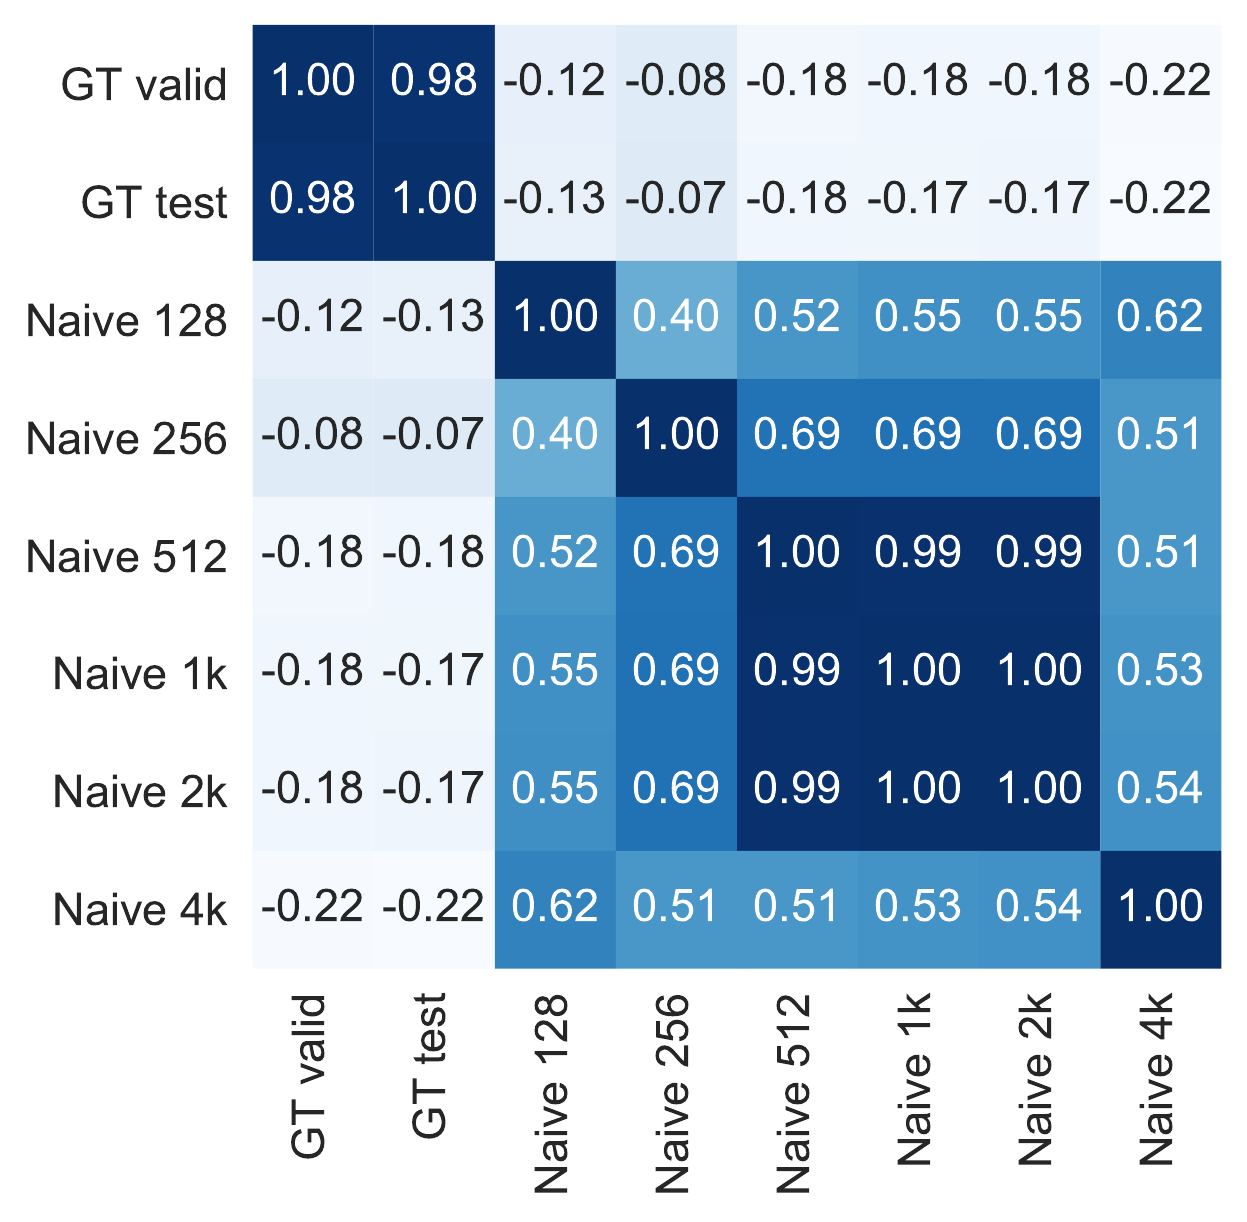}
        \caption{DARTS-PTB}
    \end{subfigure}
    \begin{subfigure}{.48\textwidth}
        \centering
        \includegraphics[width=\textwidth]{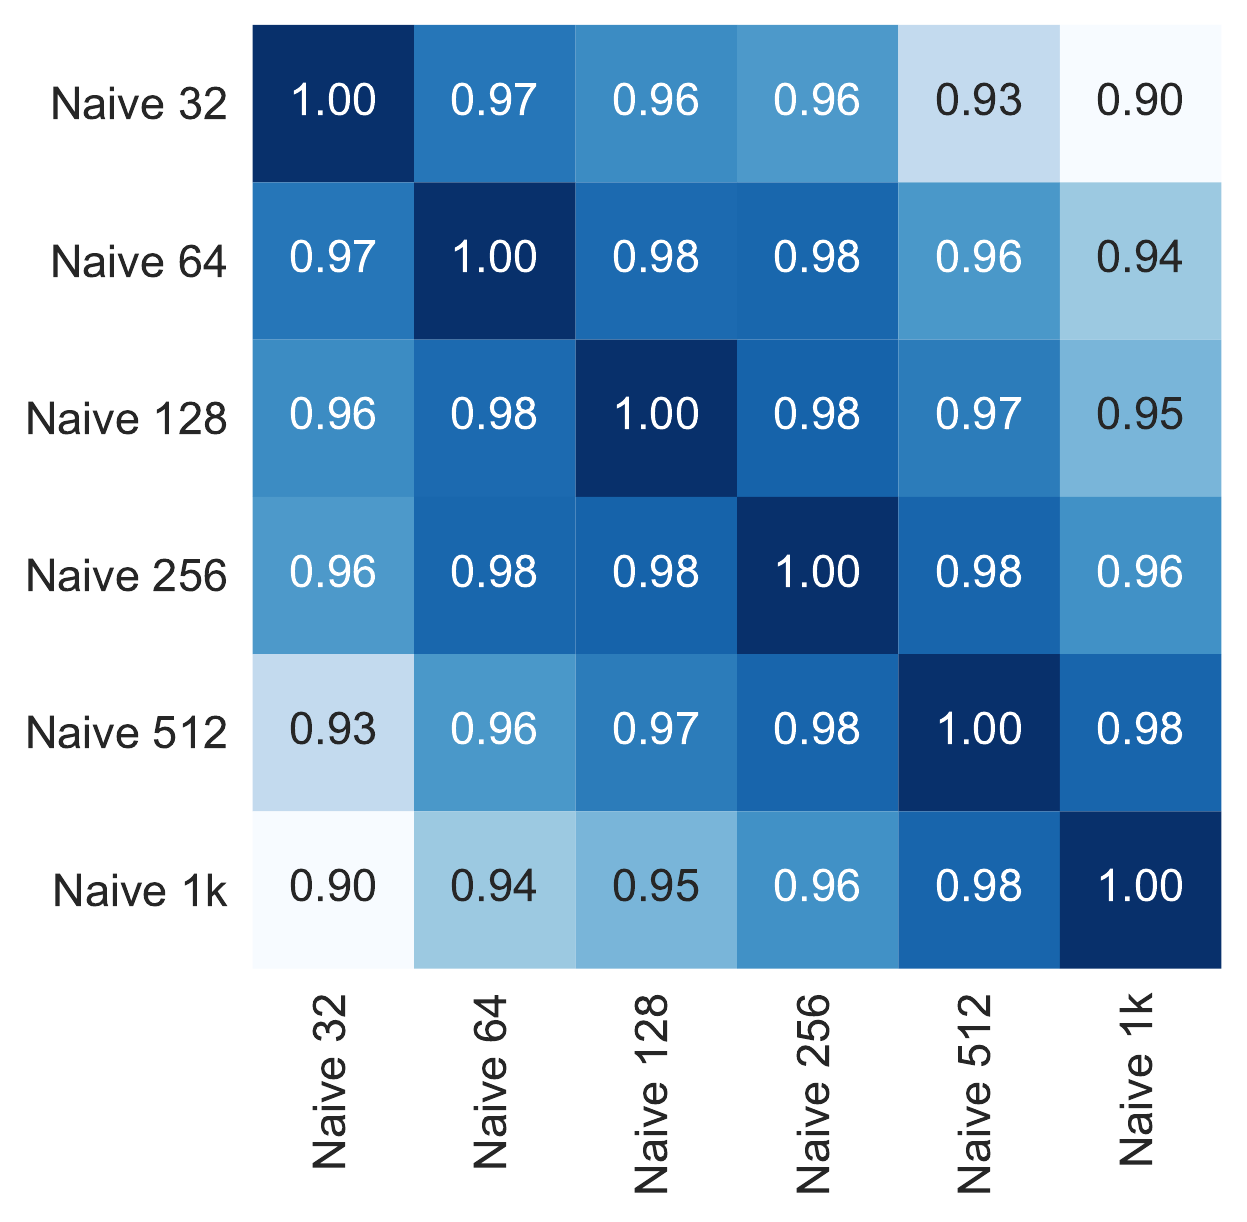}
        \caption{ProxylessNAS}
    \end{subfigure}
    \begin{subfigure}{.48\textwidth}
        \centering
        \includegraphics[width=\textwidth]{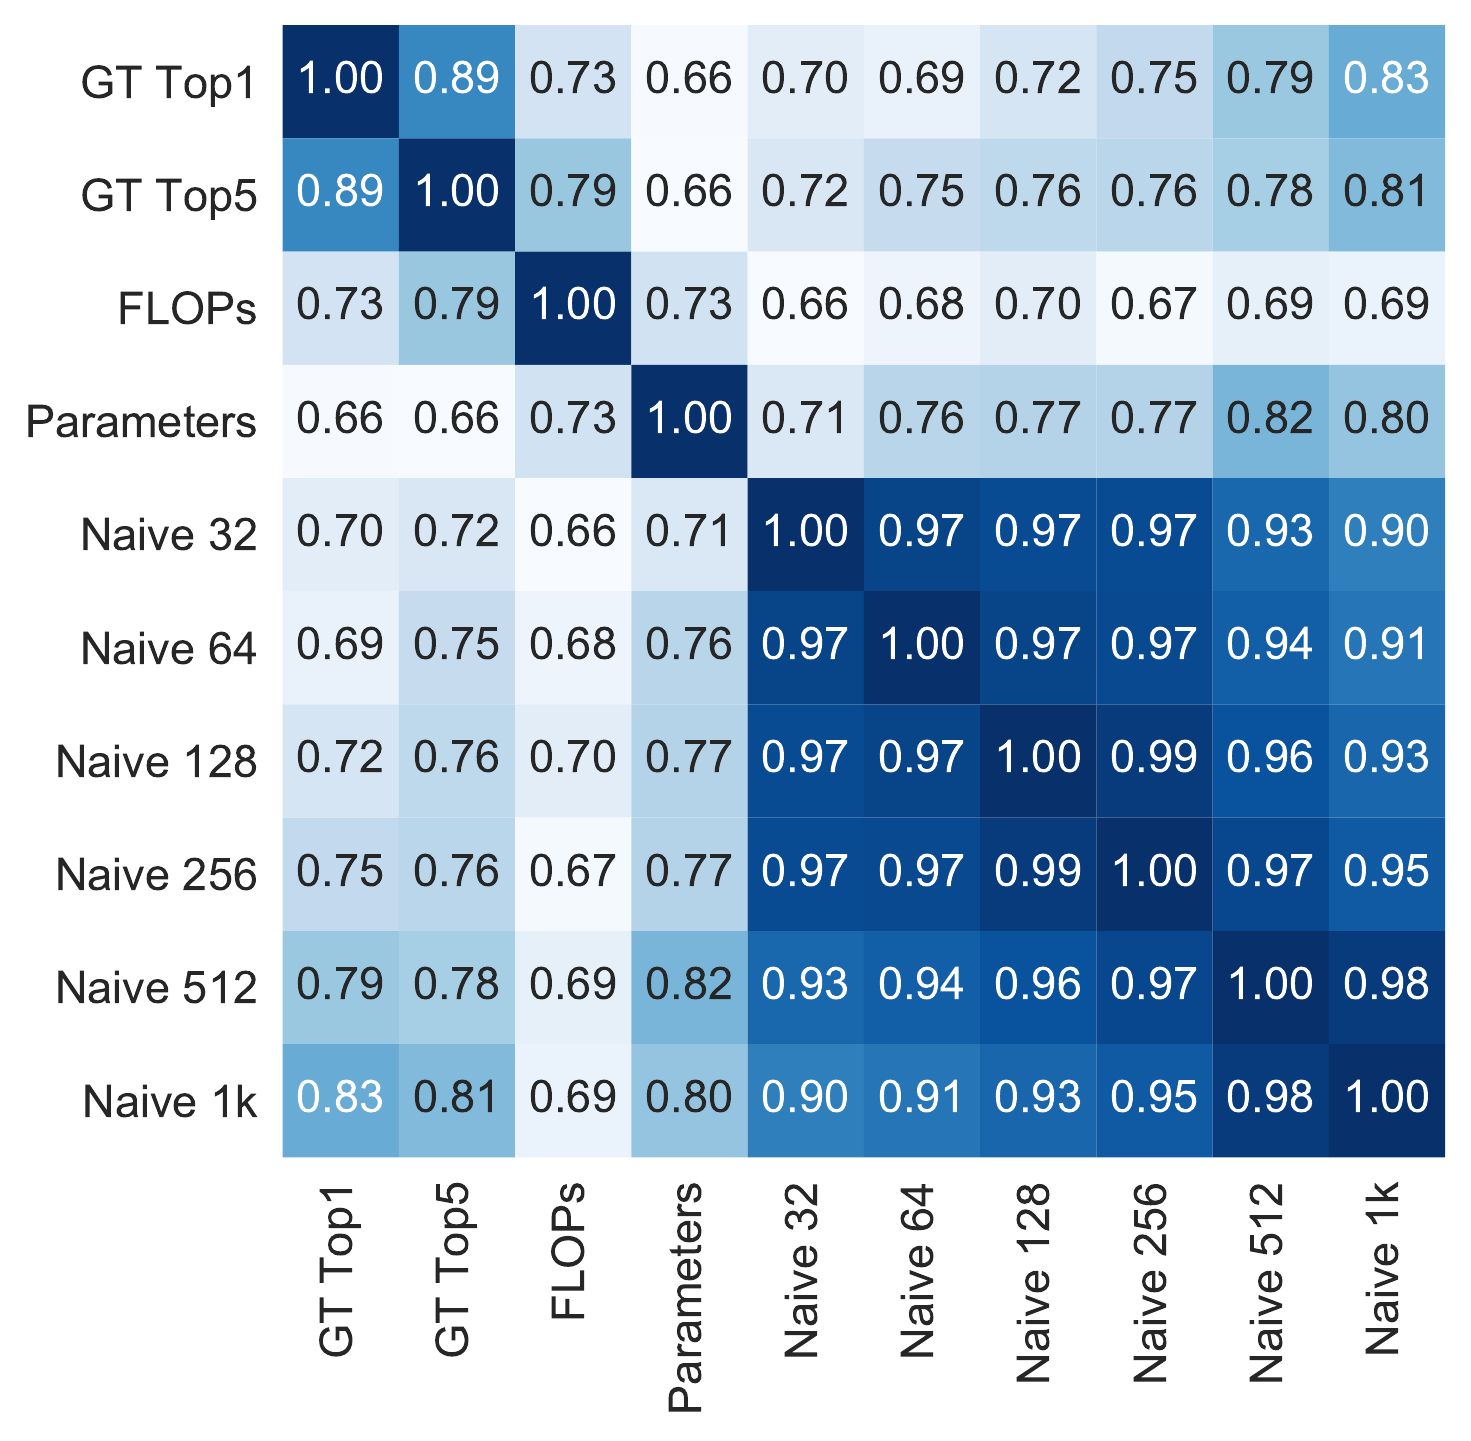}
        \caption{ProxylessNAS (FLLOPs < 600M)}
    \end{subfigure}
    \caption{Mutual correlations of all trained supernets and ground truths on various search spaces}
    \label{fig:all-correlation-others}
\end{figure}

\begin{figure}[htbp]
    \centering
    \begin{subfigure}{.48\textwidth}
        \centering
        \includegraphics[width=\textwidth]{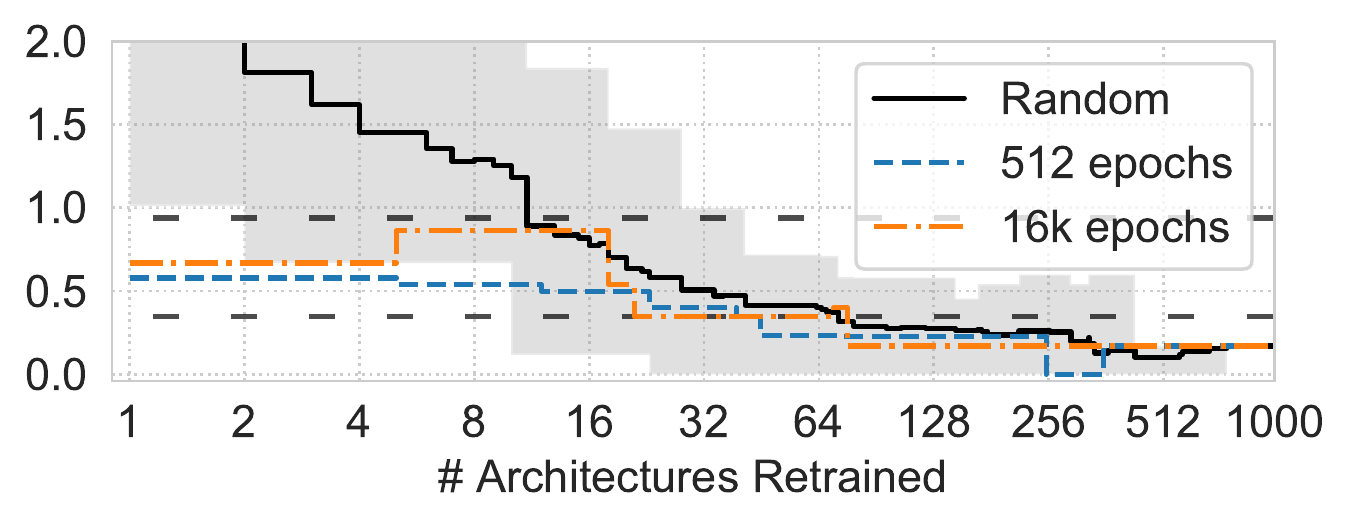}
        \caption{NAS-Bench-101}
    \end{subfigure}
    \begin{subfigure}{.48\textwidth}
        \centering
        \includegraphics[width=\textwidth]{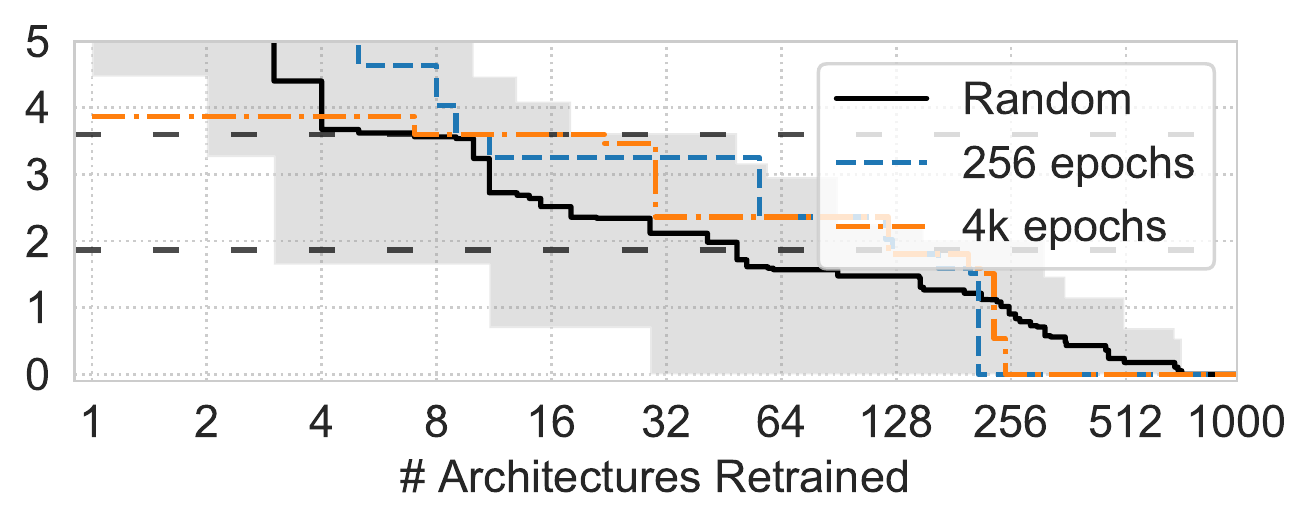}
        \caption{NAS-Bench-201}
    \end{subfigure}
    \begin{subfigure}{.48\textwidth}
        \centering
        \includegraphics[width=\textwidth]{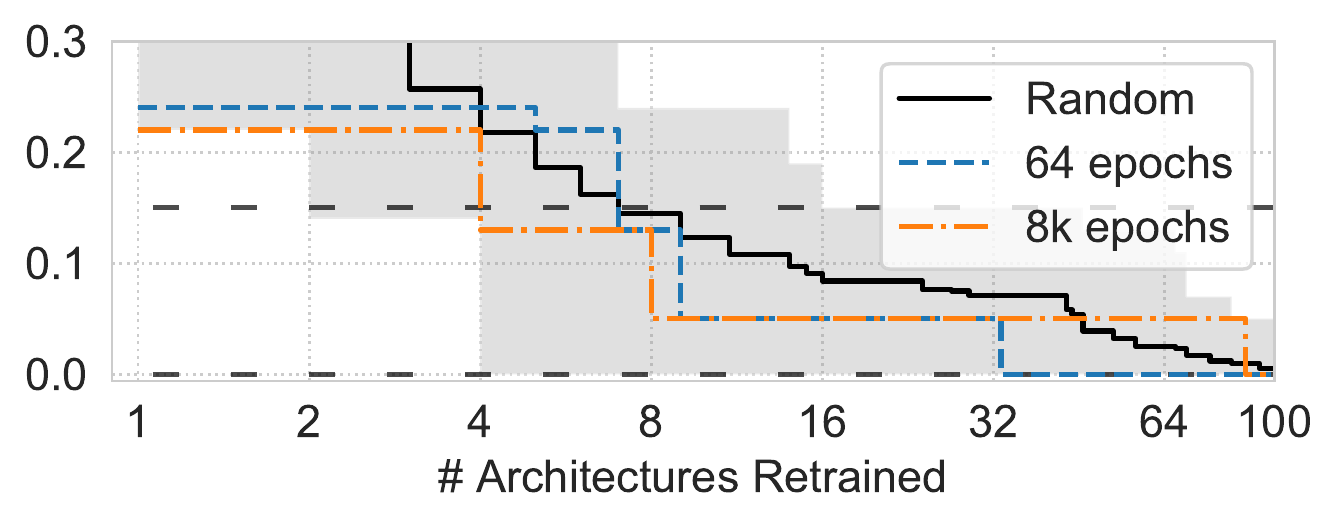}
        \caption{DARTS-CIFAR10}
    \end{subfigure}
    \begin{subfigure}{.48\textwidth}
        \centering
        \includegraphics[width=\textwidth]{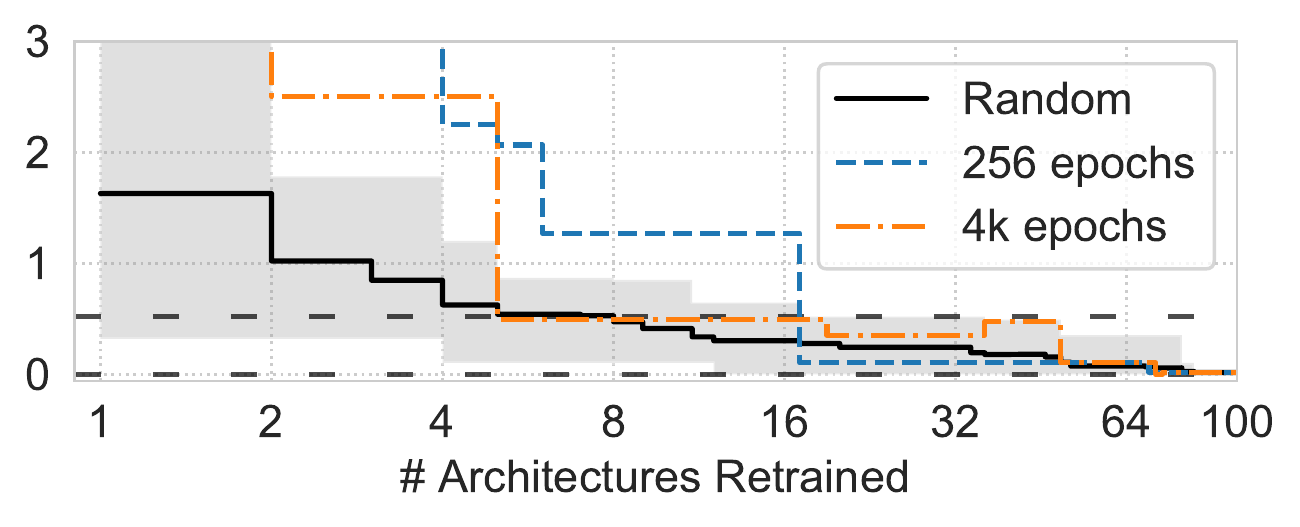}
        \caption{DARTS-PTB}
    \end{subfigure}
    \caption{Test regret~\cite{zela2020nasbench1shot1,pourchot2020share} with respect to number of retrained architectures, i.e., the test performance of the architecture with best validation performance so far compared to the ground truth best. Colored lines are two selected supernets, while the black line and the shaded region are the mean of random search and variance of random search respectively. We use two dashed lines to represent the bar of top-1\% and top-10\% respectively. As observed in the charts, supernet has little advantage compared to the random baseline when over 10 architectures have been retrained.}
    \label{fig:test-regret}
\end{figure}

\begin{figure}[htbp]
    \centering
    \begin{subfigure}{.4\textwidth}
        \centering
        \includegraphics[width=\textwidth]{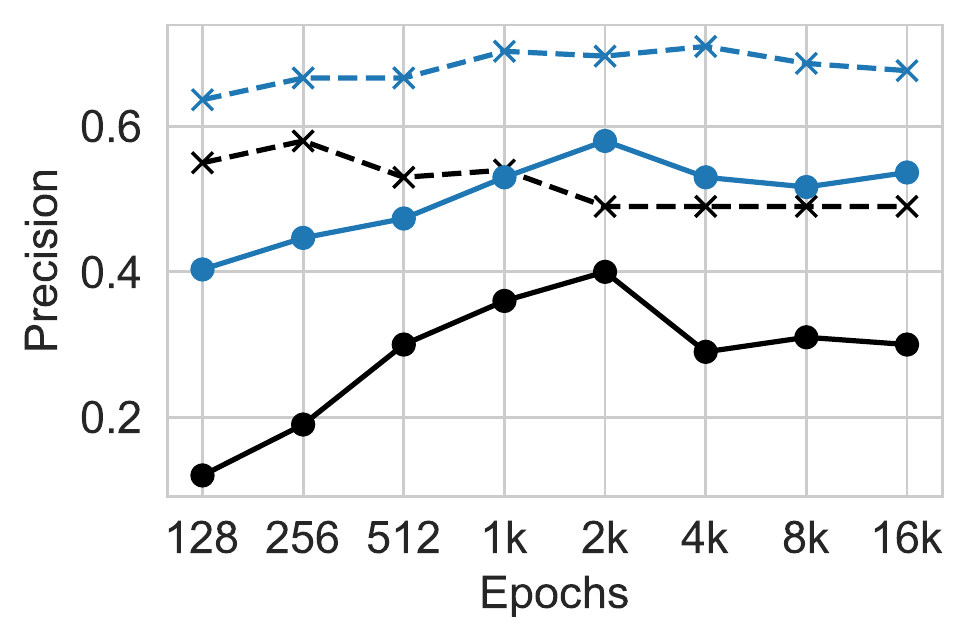}
        \caption{NAS-Bench-101}
    \end{subfigure}
    \begin{subfigure}{.4\textwidth}
        \centering
        \includegraphics[width=\textwidth]{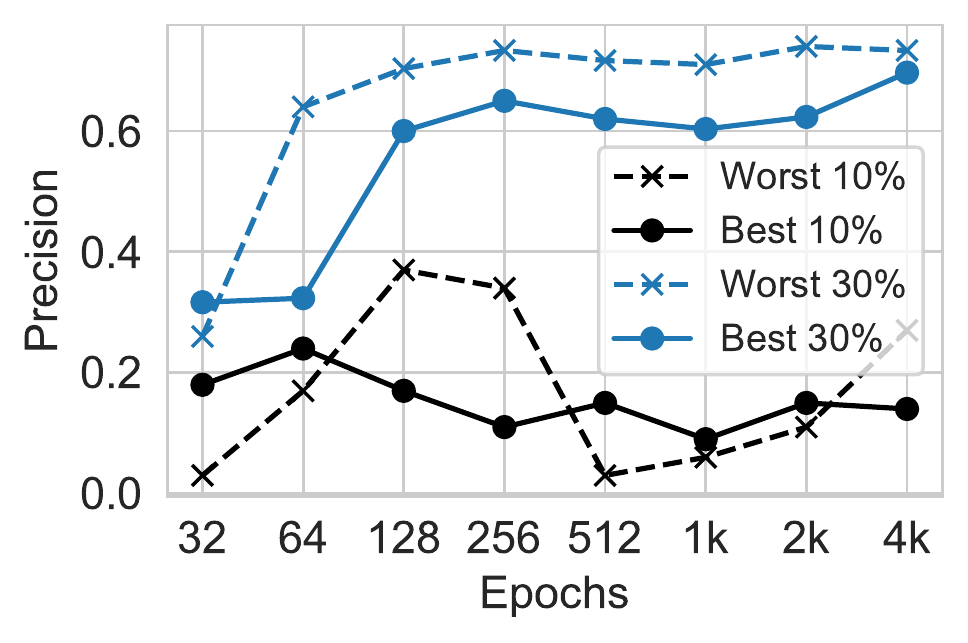}
        \caption{NAS-Bench-201}
    \end{subfigure}
    \begin{subfigure}{.4\textwidth}
        \centering
        \includegraphics[width=\textwidth]{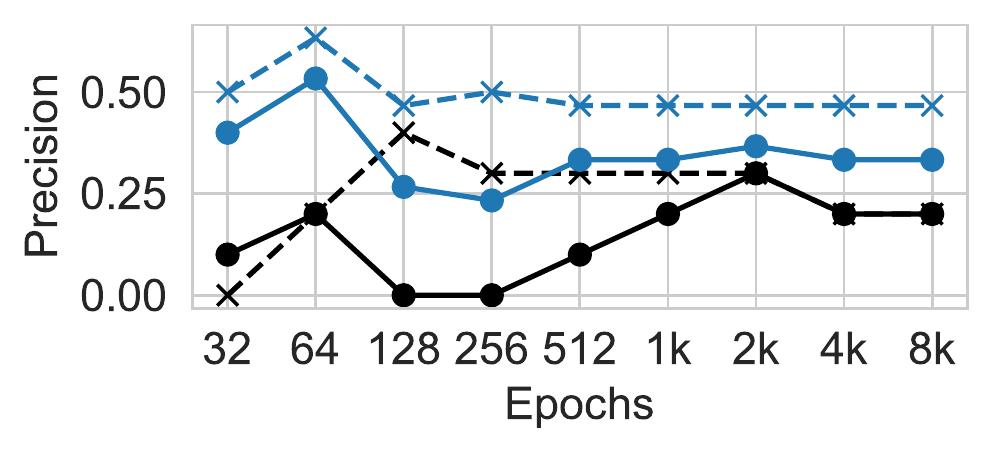}
        \caption{DARTS-CIFAR10}
    \end{subfigure}
    \begin{subfigure}{.4\textwidth}
        \centering
        \includegraphics[width=\textwidth]{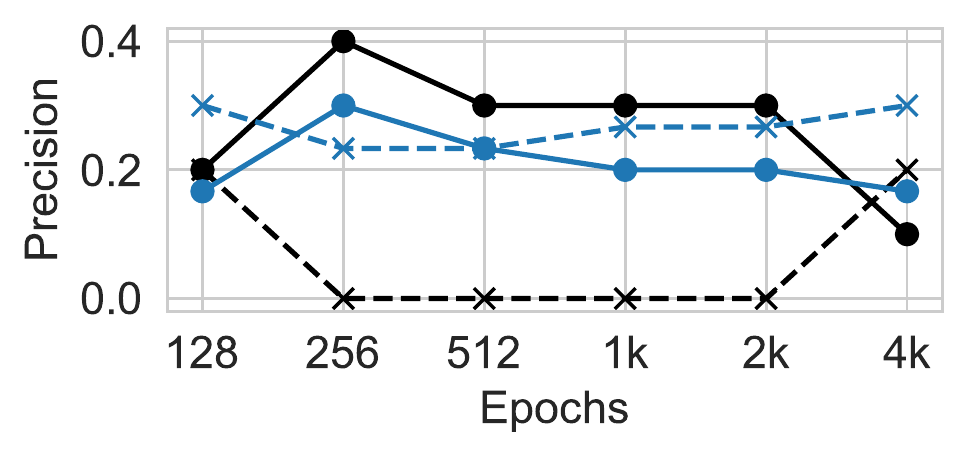}
        \caption{DARTS-PTB}
    \end{subfigure}
    \caption{Precision of best architectures and worst architectures, i.e., the overlapping ratio of the best/worst architectures between supernet performance and ground truth. We try 10\% and 30\% for the criterion of best or worst, respectively.}
    \label{fig:worst-to-best}
\end{figure}

\begin{figure}[htbp]
    \centering
    \begin{subfigure}{.9\textwidth}
        \centering
        \includegraphics[width=\textwidth]{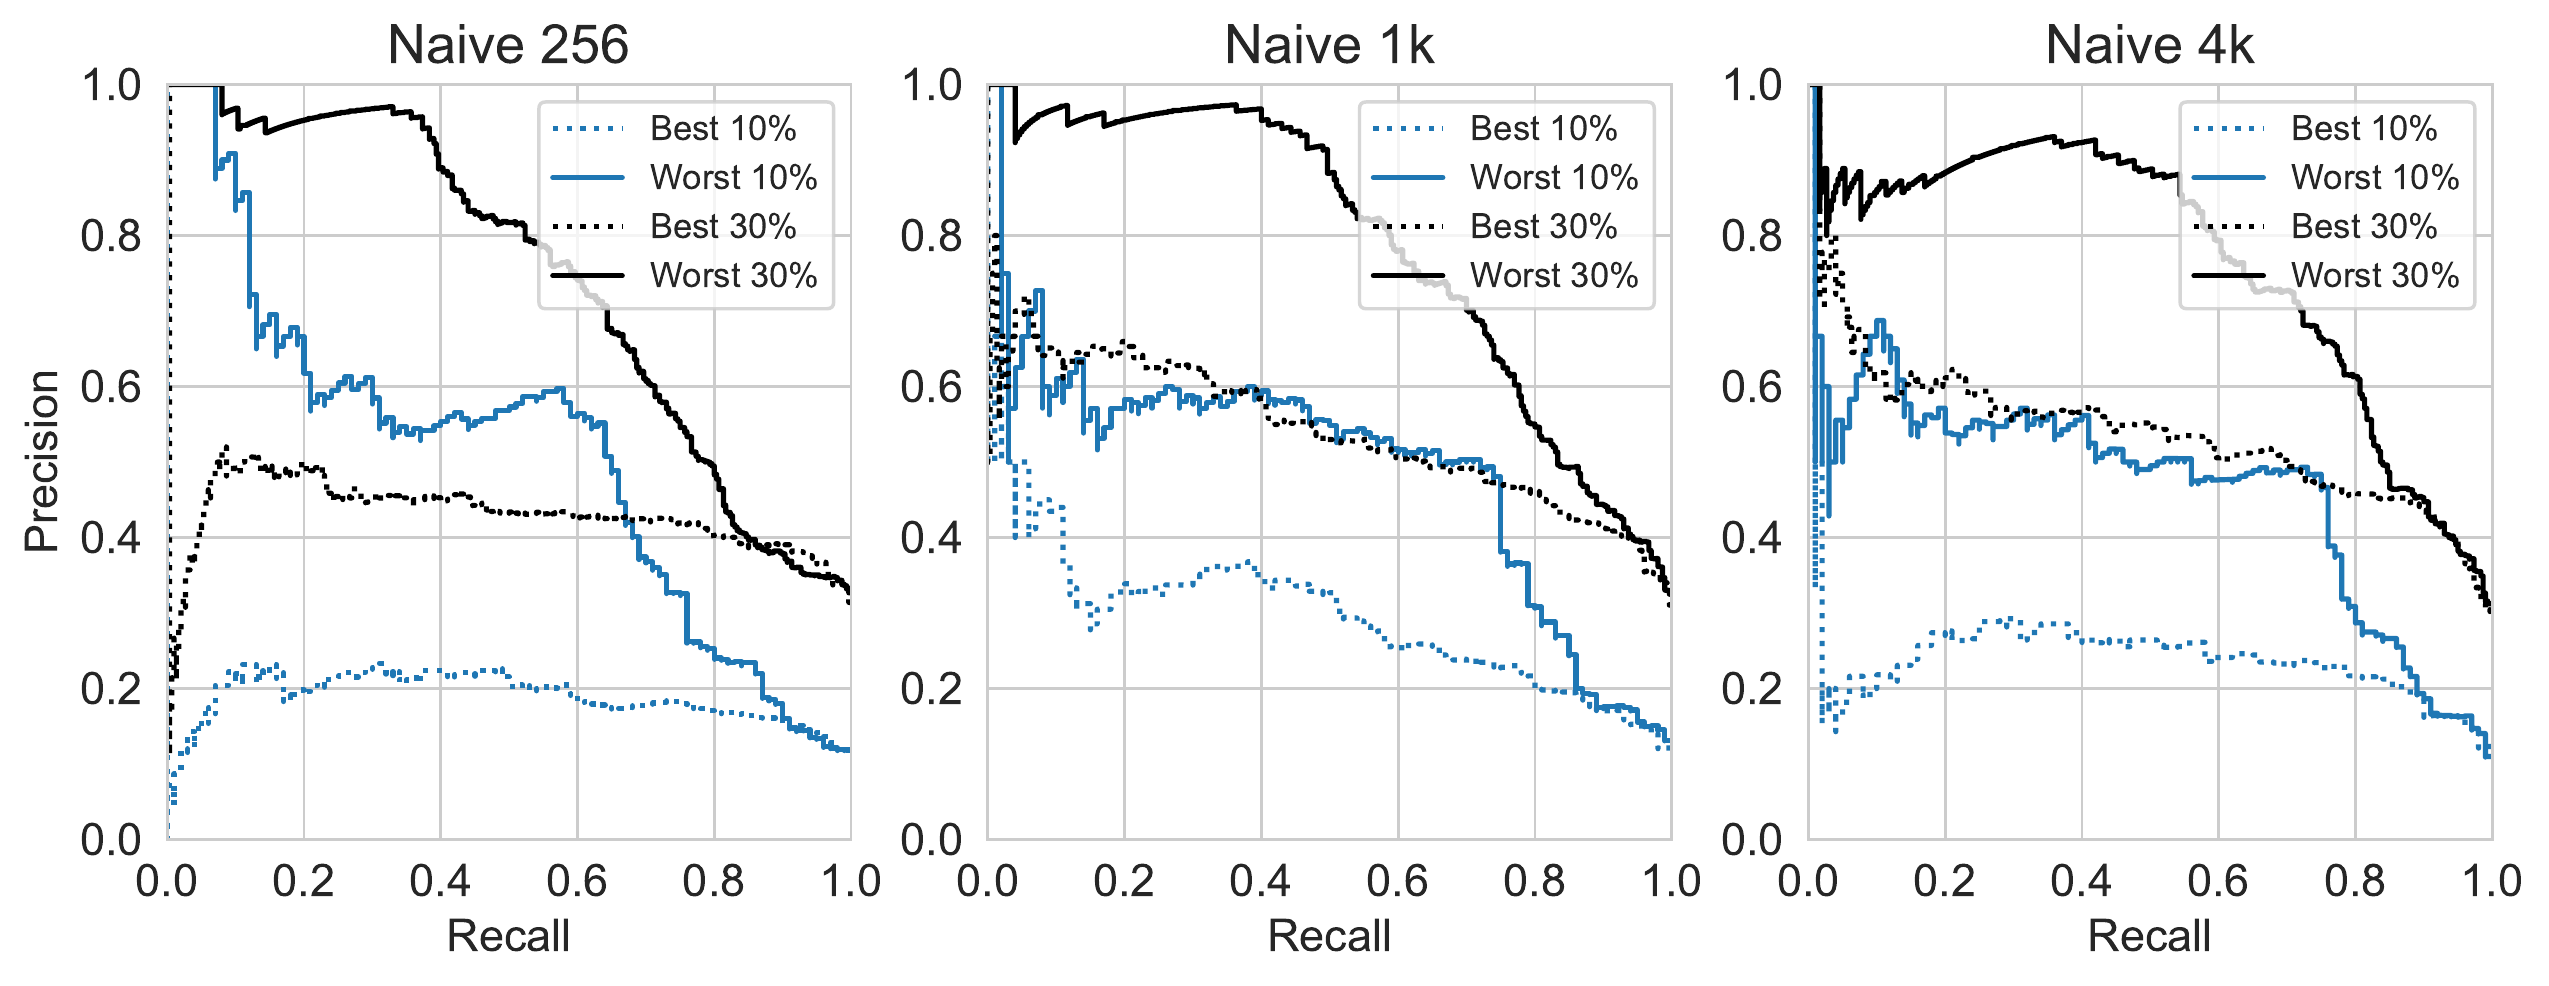}
        \caption{NAS-Bench-101}
    \end{subfigure}
    \begin{subfigure}{.9\textwidth}
        \centering
        \includegraphics[width=\textwidth]{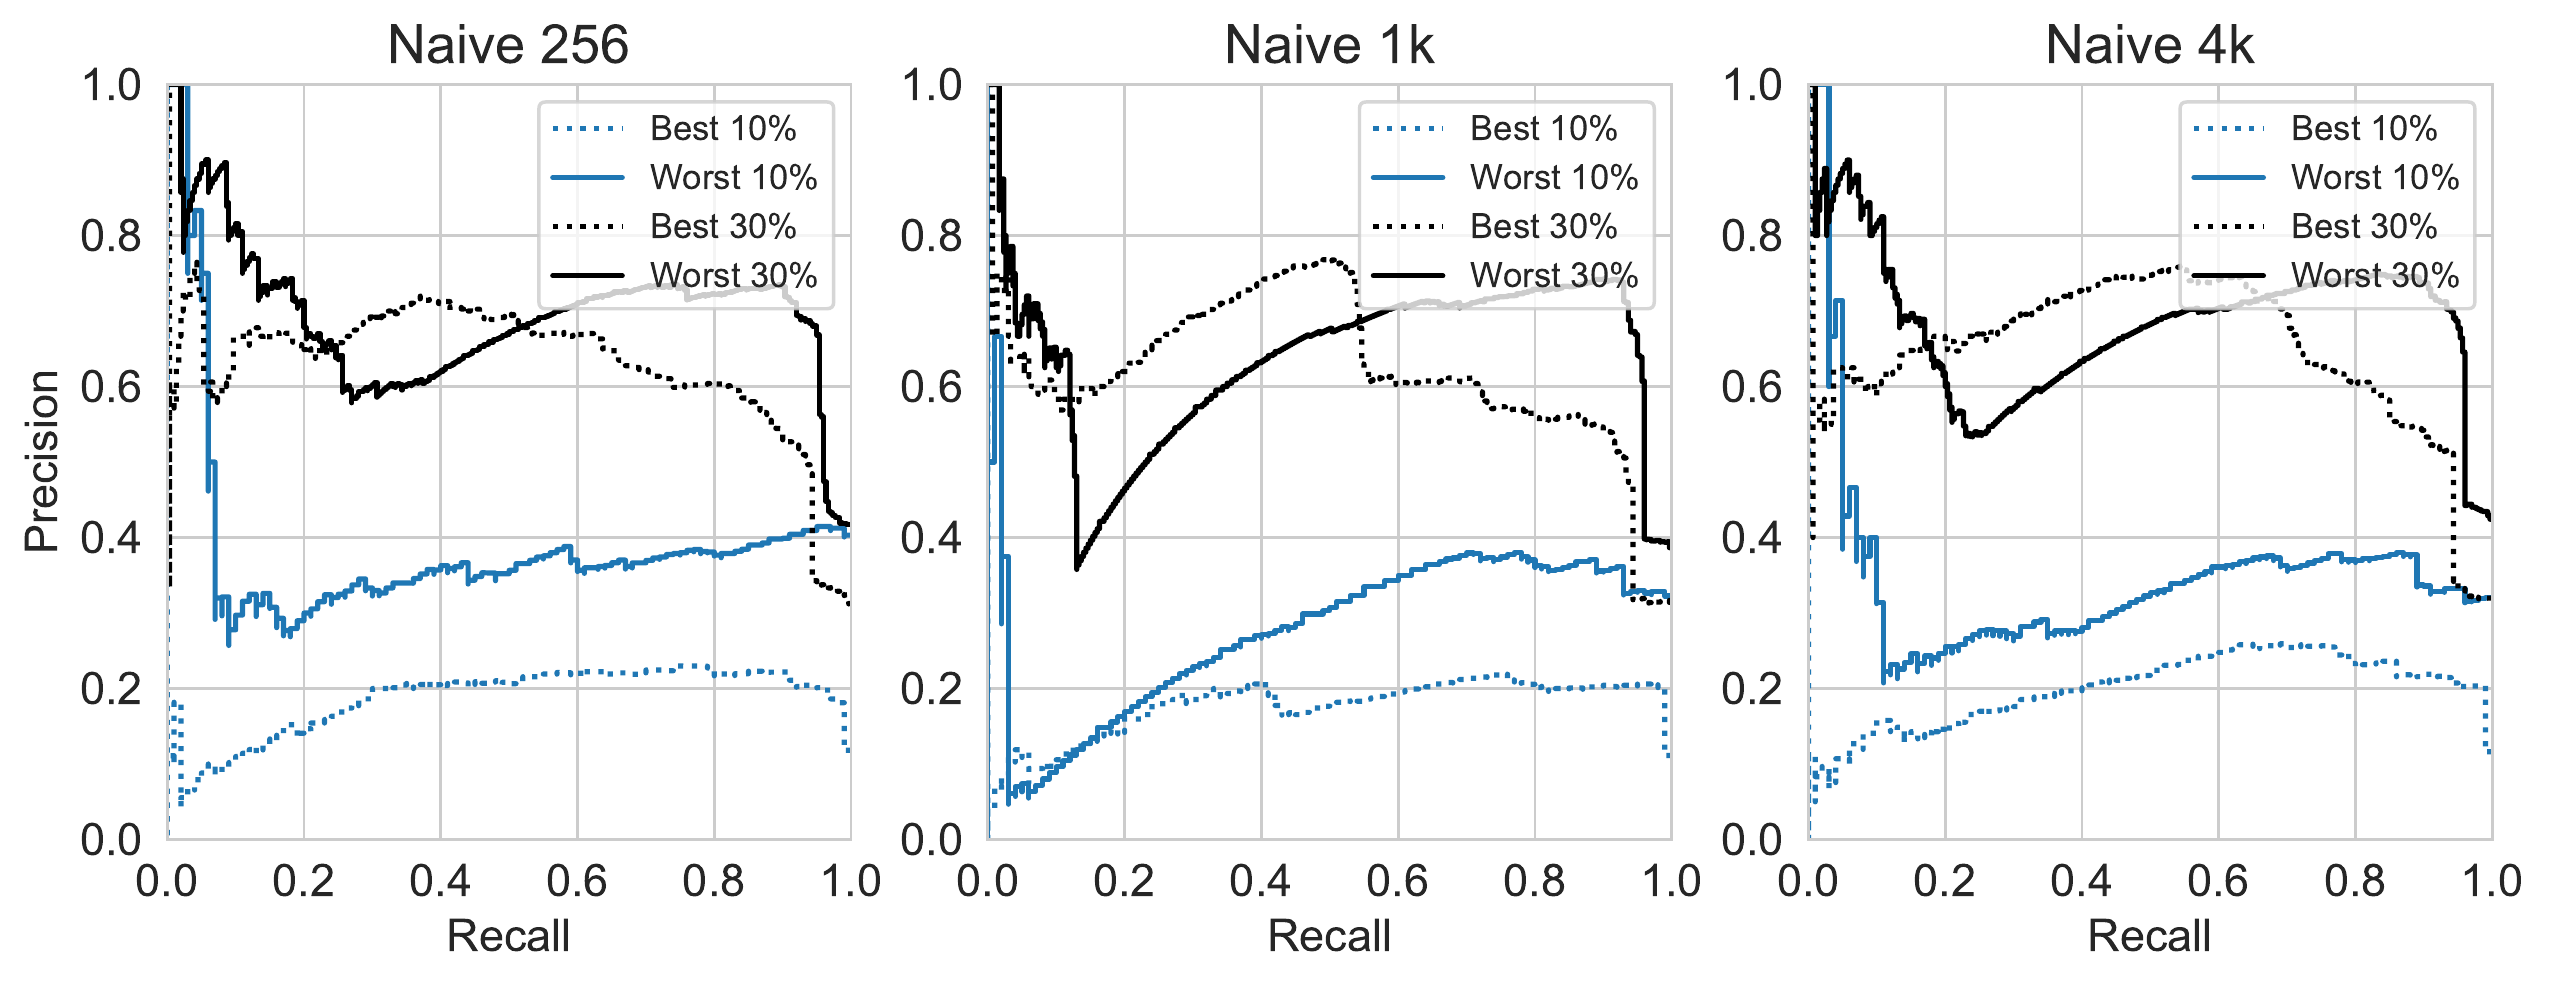}
        \caption{NAS-Bench-201}
    \end{subfigure}
    \begin{subfigure}{.9\textwidth}
        \centering
        \includegraphics[width=\textwidth]{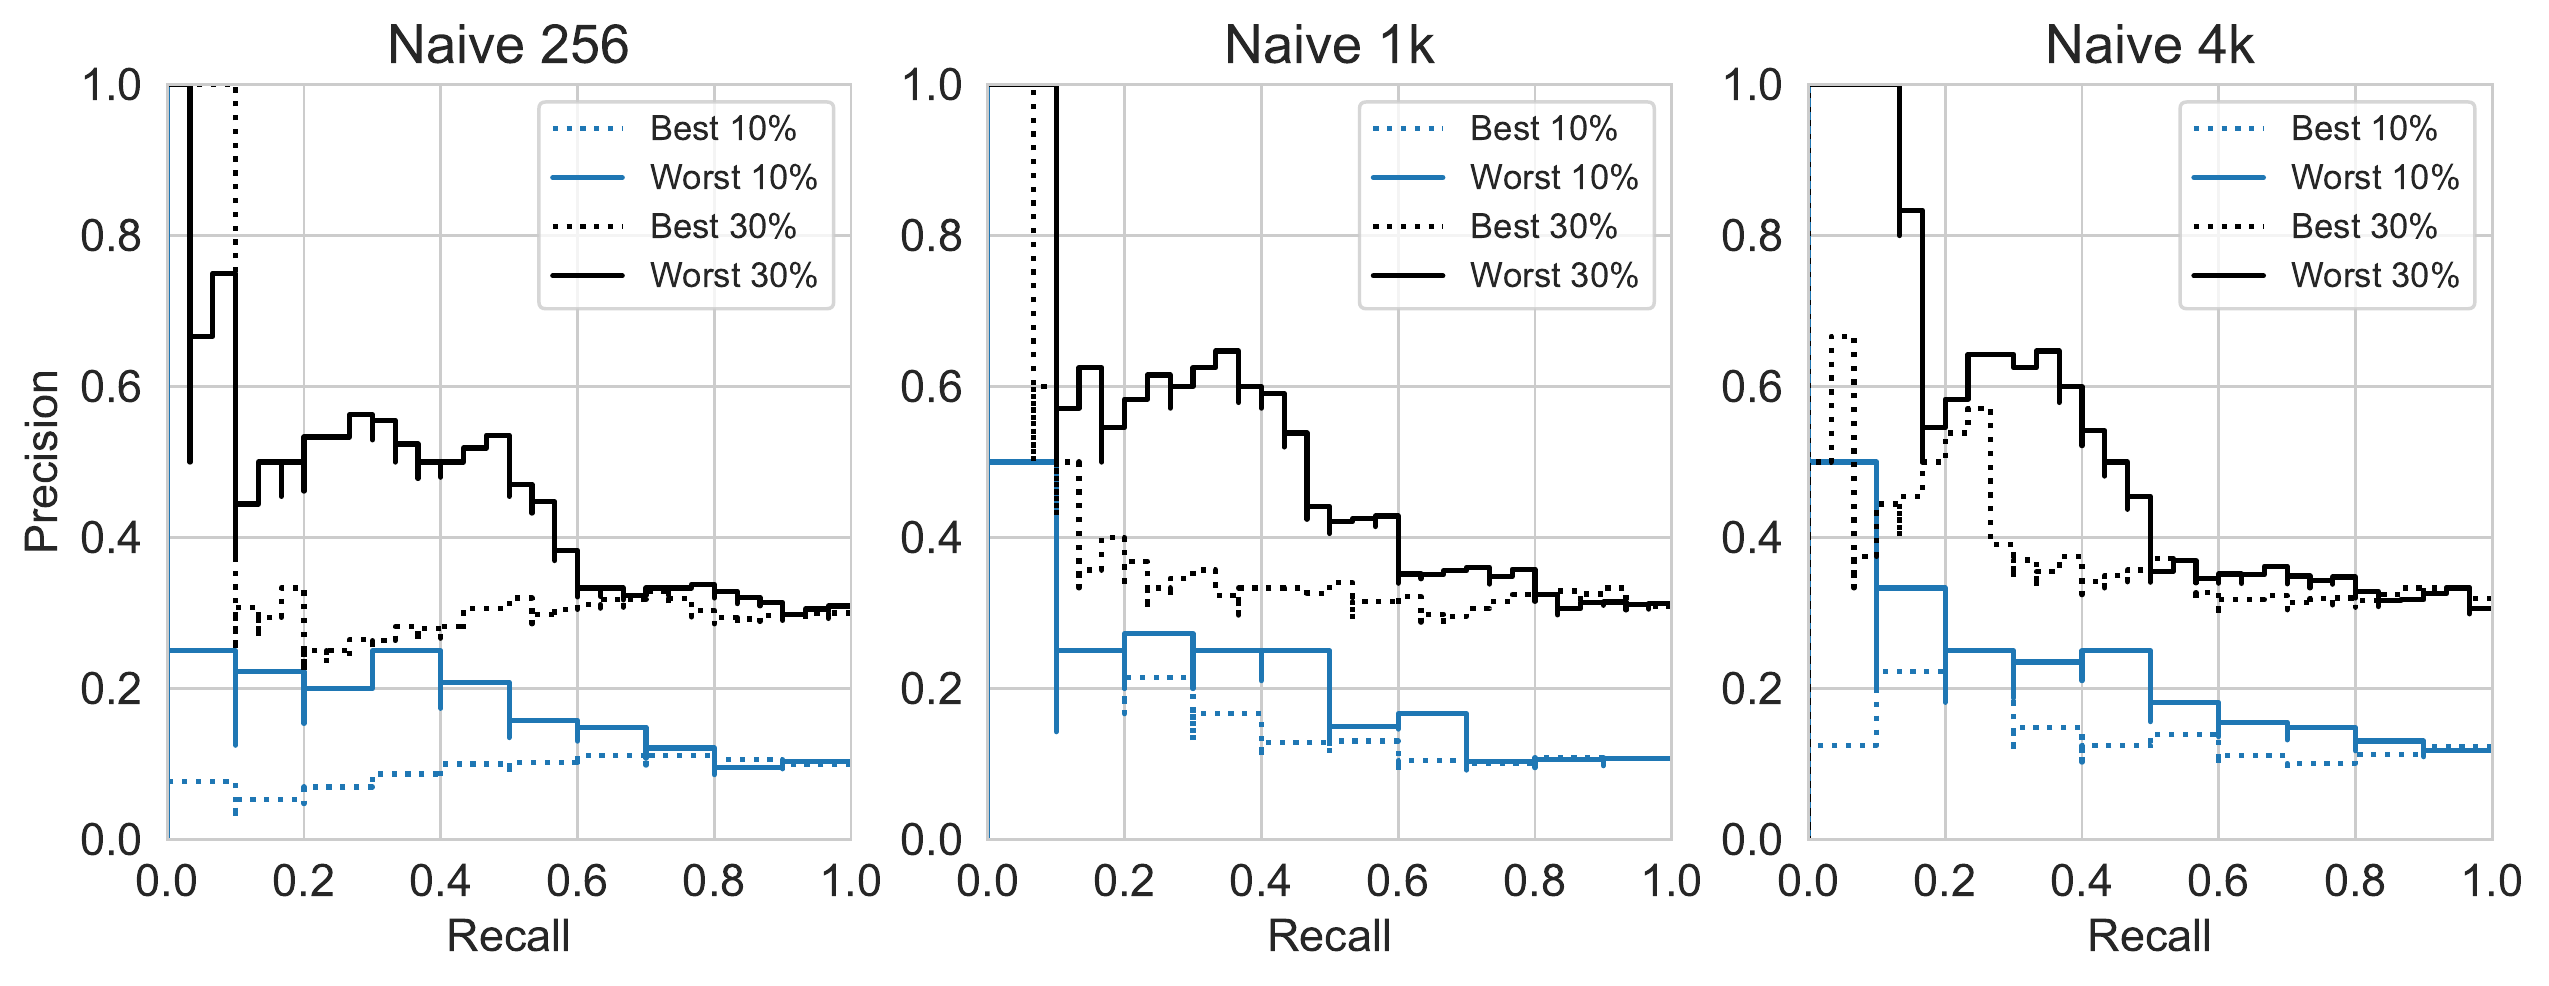}
        \caption{DARTS-CIFAR10}
    \end{subfigure}
    \begin{subfigure}{.9\textwidth}
        \centering
        \includegraphics[width=\textwidth]{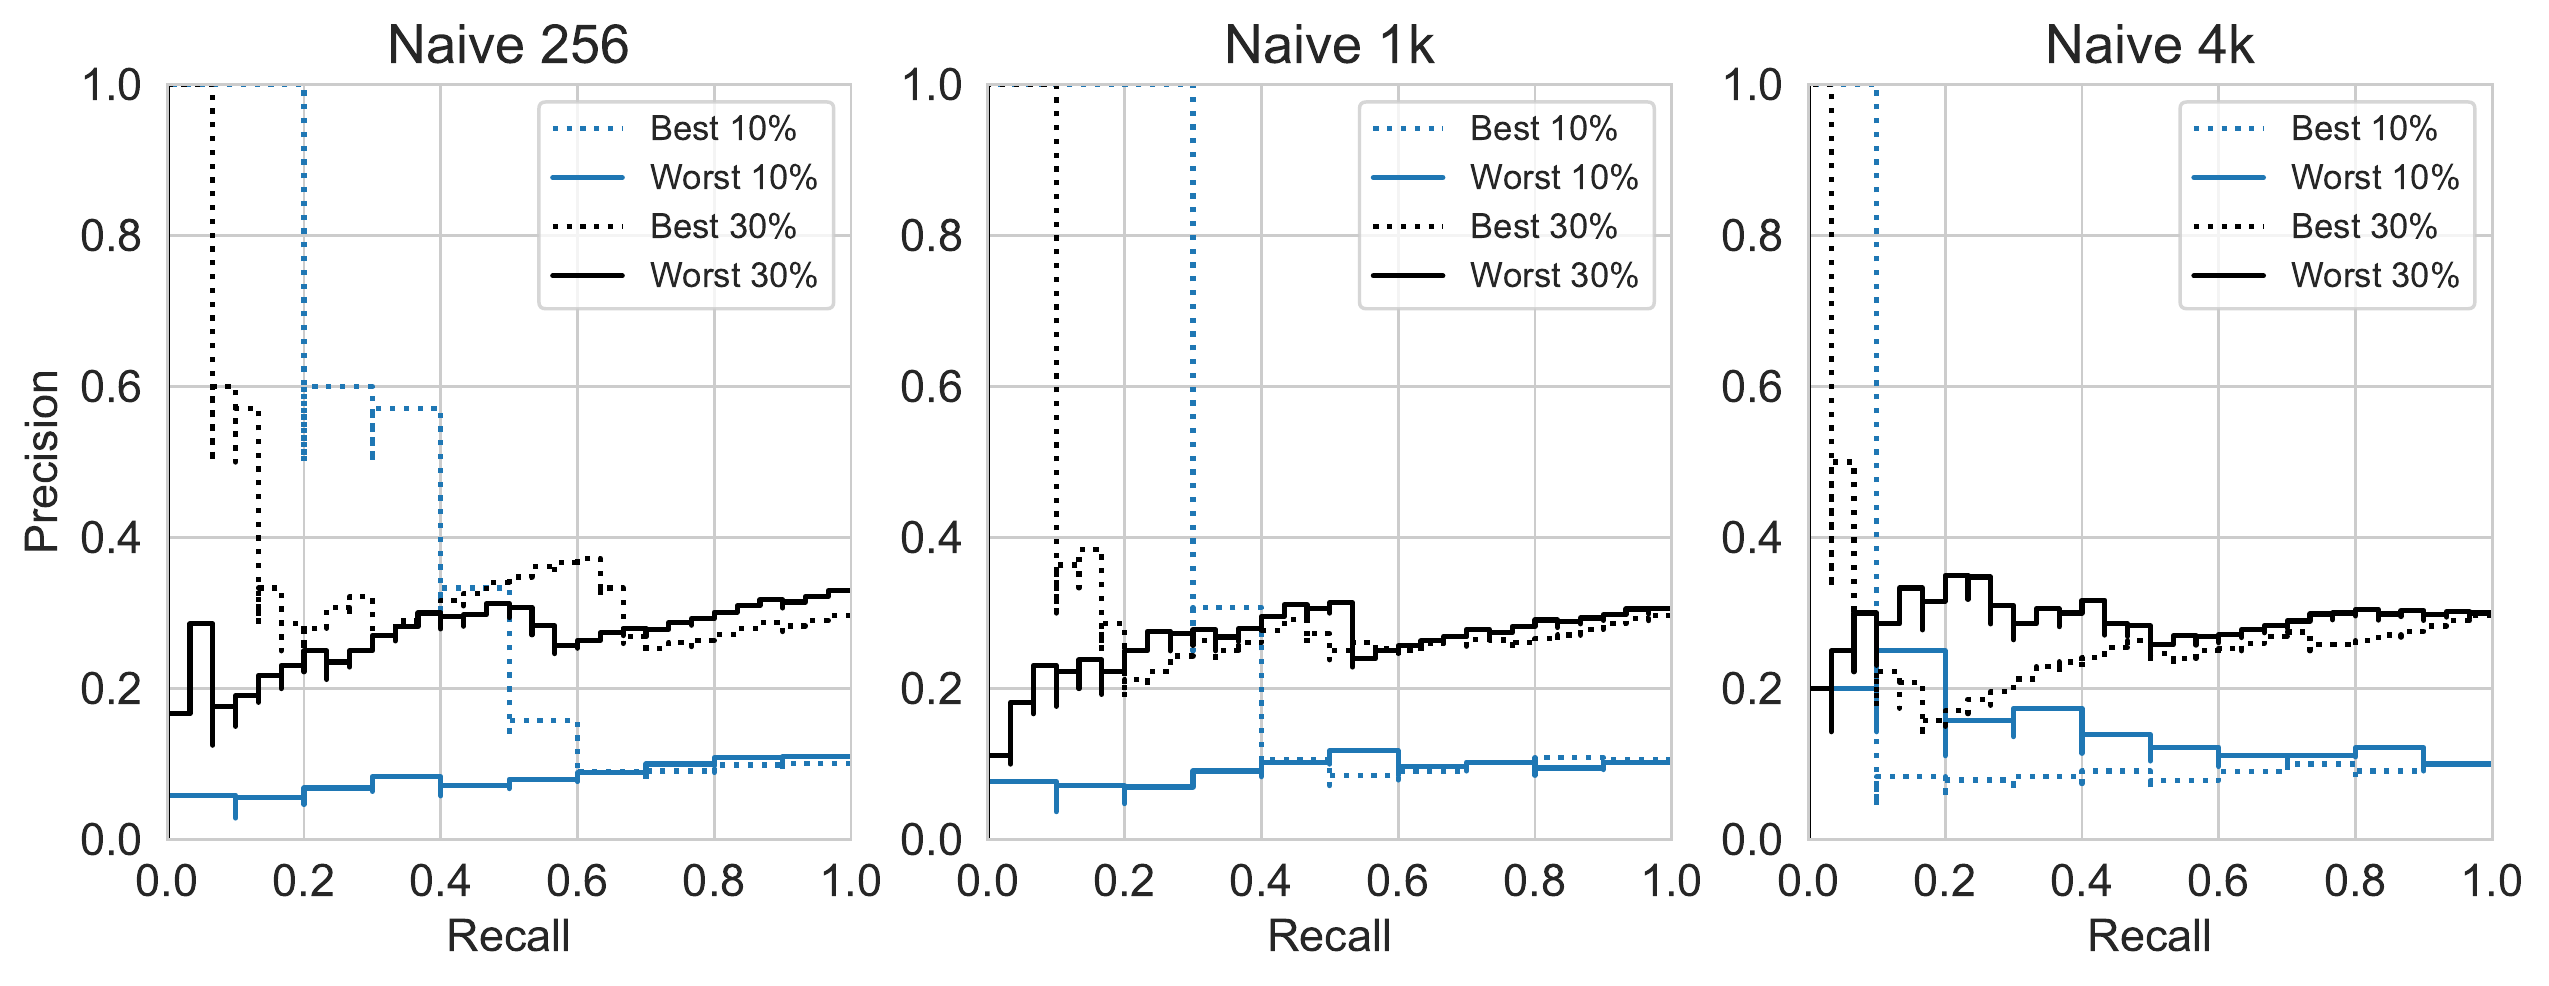}
        \caption{DARTS-PTB}
    \end{subfigure}
    \caption{Precision-recall of best architectures and worst architectures, similar to the setups of \autoref{fig:worst-to-best}. Architectures are examined from worst to best in the ``worst'' scenario, and from best to worst in the ``best'' scenario.}
\end{figure}

% \section{Proofs}

% \subsection{Estimating Random Baseline of Top-k}

% Suppose we have $n$ architectures and their ground truth performances are $p_1, p_2, \ldots, p_n$ respectively, where $p_1 < p_2 < \cdots < p_n$. The higher the better. We then randomly sample $k$ architectures. The expectation of the best performance of these $k$ architectures is:

% \begin{equation}
%     \frac{1}{\binom{n}{k}} \sum_{i=k}^n \binom{i-1}{k-1} p_k
% \end{equation}

% which can be computed in $\mathcal{O}(n)$ time with expansion and factorization tricks.
